# Supplementary material for: MAVRL: Learning Reward Functions from Multiple Feedback Types with Amortized Variational Inference
Source: arXiv:2602.15206 source file (2026-06-19)
Supplement: Supplementary file 1 [file appendix-in-distribution-full.tex]

\section{Additional In-Distribution Results}
\label{sec:appendix-in-distribution}
We report performance results for all tested feedback budgets in \cref{tab:appendix_grid_cliff}, \cref{tab:appendix_grid_sparse}, \cref{tab:appendix_grid_trap}, \cref{tab:appendix_cartpole_v1}, \cref{tab:appendix_acrobot_v1}, and \cref{tab:appendix_lunarlander_v3}.

% Requires: \usepackage{booktabs}
\begin{table}[htbp]
\centering
\small
\caption{Full results for Grid Cliff (normalized discounted value, higher is better)}
\label{tab:appendix_grid_cliff}
\begin{tabular}{lrrrr|rrrrrr|r}
\toprule
 & \multicolumn{4}{c|}{Singles} & \multicolumn{6}{c|}{Pairs} & \multicolumn{1}{c}{All} \\
Budget (P,D,R,S) & \fbPref & \fbDemo & \fbRating & \fbStop & \fbDemoPref & \fbPrefRating & \fbPrefStop & \fbDemoRating & \fbDemoStop & \fbRatingStop & \fbPDRS \\
\midrule
(64, 1, 32, 128) & 20.4 & \textbf{62.6} & 19.9 & 8.4 & 16.3 & 27.6 & 38.1 & 32.8 & 56.1 & 29.8 & 51.5 \\
(64, 1, 32, 256) & 20.4 & 62.6 & 19.9 & 37.4 & 16.3 & 27.6 & 60.3 & 32.8 & 72.2 & 63.4 & \textbf{77.8} \\
(64, 1, 64, 128) & 20.4 & 62.6 & 41.3 & 8.4 & 16.3 & 49.5 & 38.1 & 41.8 & 56.1 & 48.6 & \textbf{64.7} \\
(64, 1, 64, 256) & 20.4 & 62.6 & 41.3 & 37.4 & 16.3 & 49.5 & 60.3 & 41.8 & 72.2 & 72.8 & \textbf{90.8} \\
(64, 1, 128, 128) & 20.4 & 62.6 & 75.0 & 8.4 & 16.3 & 73.3 & 38.1 & 63.6 & 56.1 & 59.6 & \textbf{86.6} \\
(64, 1, 128, 256) & 20.4 & 62.6 & 75.0 & 37.4 & 16.3 & 73.3 & 60.3 & 63.6 & 72.2 & 85.6 & \textbf{91.0} \\
(64, 2, 32, 128) & 20.4 & 32.0 & 19.9 & 8.4 & 3.6 & 27.6 & 38.1 & 21.7 & \textbf{52.4} & 29.8 & 39.7 \\
(64, 2, 32, 256) & 20.4 & 32.0 & 19.9 & 37.4 & 3.6 & 27.6 & 60.3 & 21.7 & 72.2 & 63.4 & \textbf{82.3} \\
(64, 2, 64, 128) & 20.4 & 32.0 & 41.3 & 8.4 & 3.6 & 49.5 & 38.1 & 37.6 & \textbf{52.4} & 48.6 & 47.1 \\
(64, 2, 64, 256) & 20.4 & 32.0 & 41.3 & 37.4 & 3.6 & 49.5 & 60.3 & 37.6 & 72.2 & 72.8 & \textbf{86.6} \\
(64, 2, 128, 128) & 20.4 & 32.0 & 75.0 & 8.4 & 3.6 & 73.3 & 38.1 & 73.6 & 52.4 & 59.6 & \textbf{82.2} \\
(64, 2, 128, 256) & 20.4 & 32.0 & 75.0 & 37.4 & 3.6 & 73.3 & 60.3 & 73.6 & 72.2 & 85.6 & \textbf{95.5} \\
(128, 1, 32, 128) & 29.7 & \textbf{62.6} & 19.9 & 8.4 & 29.7 & 38.5 & 38.5 & 32.8 & 56.1 & 29.8 & 51.6 \\
(128, 1, 32, 256) & 29.7 & 62.6 & 19.9 & 37.4 & 29.7 & 38.5 & 60.3 & 32.8 & \textbf{72.2} & 63.4 & 69.0 \\
(128, 1, 64, 128) & 29.7 & \textbf{62.6} & 41.3 & 8.4 & 29.7 & 47.2 & 38.5 & 41.8 & 56.1 & 48.6 & 56.0 \\
(128, 1, 64, 256) & 29.7 & 62.6 & 41.3 & 37.4 & 29.7 & 47.2 & 60.3 & 41.8 & 72.2 & 72.8 & \textbf{73.4} \\
(128, 1, 128, 128) & 29.7 & 62.6 & \textbf{75.0} & 8.4 & 29.7 & 56.0 & 38.5 & 63.6 & 56.1 & 59.6 & 55.9 \\
(128, 1, 128, 256) & 29.7 & 62.6 & 75.0 & 37.4 & 29.7 & 56.0 & 60.3 & 63.6 & 72.2 & \textbf{85.6} & 82.2 \\
(128, 2, 32, 128) & 29.7 & 32.0 & 19.9 & 8.4 & 29.6 & 38.5 & 38.5 & 21.7 & \textbf{52.4} & 29.8 & 42.9 \\
(128, 2, 32, 256) & 29.7 & 32.0 & 19.9 & 37.4 & 29.6 & 38.5 & 60.3 & 21.7 & \textbf{72.2} & 63.4 & 69.0 \\
(128, 2, 64, 128) & 29.7 & 32.0 & 41.3 & 8.4 & 29.6 & 47.2 & 38.5 & 37.6 & 52.4 & 48.6 & \textbf{56.0} \\
(128, 2, 64, 256) & 29.7 & 32.0 & 41.3 & 37.4 & 29.6 & 47.2 & 60.3 & 37.6 & 72.2 & 72.8 & \textbf{77.9} \\
(128, 2, 128, 128) & 29.7 & 32.0 & \textbf{75.0} & 8.4 & 29.6 & 56.0 & 38.5 & 73.6 & 52.4 & 59.6 & 56.0 \\
(128, 2, 128, 256) & 29.7 & 32.0 & 75.0 & 37.4 & 29.6 & 56.0 & 60.3 & 73.6 & 72.2 & 85.6 & \textbf{86.7} \\
(256, 1, 32, 128) & 60.5 & 62.6 & 19.9 & 8.4 & 64.9 & \textbf{69.3} & 60.4 & 32.8 & 56.1 & 29.8 & 69.2 \\
(256, 1, 32, 256) & 60.5 & 62.6 & 19.9 & 37.4 & 64.9 & 69.3 & 73.6 & 32.8 & 72.2 & 63.4 & \textbf{82.3} \\
(256, 1, 64, 128) & 60.5 & 62.6 & 41.3 & 8.4 & 64.9 & 69.3 & 60.4 & 41.8 & 56.1 & 48.6 & \textbf{73.6} \\
(256, 1, 64, 256) & 60.5 & 62.6 & 41.3 & 37.4 & 64.9 & 69.3 & 73.6 & 41.8 & 72.2 & 72.8 & \textbf{86.7} \\
(256, 1, 128, 128) & 60.5 & 62.6 & 75.0 & 8.4 & 64.9 & 78.1 & 60.4 & 63.6 & 56.1 & 59.6 & \textbf{86.8} \\
(256, 1, 128, 256) & 60.5 & 62.6 & 75.0 & 37.4 & 64.9 & 78.1 & 73.6 & 63.6 & 72.2 & \textbf{85.6} & 82.3 \\
(256, 2, 32, 128) & 60.5 & 32.0 & 19.9 & 8.4 & 60.5 & \textbf{69.3} & 60.4 & 21.7 & 52.4 & 29.8 & \textbf{69.3} \\
(256, 2, 32, 256) & 60.5 & 32.0 & 19.9 & 37.4 & 60.5 & 69.3 & \textbf{73.6} & 21.7 & 72.2 & 63.4 & \textbf{73.6} \\
(256, 2, 64, 128) & 60.5 & 32.0 & 41.3 & 8.4 & 60.5 & 69.3 & 60.4 & 37.6 & 52.4 & 48.6 & \textbf{78.1} \\
(256, 2, 64, 256) & 60.5 & 32.0 & 41.3 & 37.4 & 60.5 & 69.3 & 73.6 & 37.6 & 72.2 & 72.8 & \textbf{82.5} \\
(256, 2, 128, 128) & 60.5 & 32.0 & 75.0 & 8.4 & 60.5 & \textbf{78.1} & 60.4 & 73.6 & 52.4 & 59.6 & \textbf{78.1} \\
(256, 2, 128, 256) & 60.5 & 32.0 & 75.0 & 37.4 & 60.5 & 78.1 & 73.6 & 73.6 & 72.2 & \textbf{85.6} & 82.5 \\
\bottomrule
\end{tabular}
\end{table}
% Requires: \usepackage{booktabs}
\begin{table}[htbp]
\centering
\small
\caption{Full results for Grid Sparse (normalized discounted value, higher is better)}
\label{tab:appendix_grid_sparse}
\begin{tabular}{lrrrr|rrrrrr|r}
\toprule
 & \multicolumn{4}{c|}{Singles} & \multicolumn{6}{c|}{Pairs} & \multicolumn{1}{c}{All} \\
Budget (P,D,R,S) & \fbPref & \fbDemo & \fbRating & \fbStop & \fbDemoPref & \fbPrefRating & \fbPrefStop & \fbDemoRating & \fbDemoStop & \fbRatingStop & \fbPDRS \\
\midrule
(64, 1, 32, 128) & 4.9 & 65.0 & 20.2 & 25.0 & -0.1 & 4.9 & 9.9 & 35.0 & \textbf{80.0} & 40.0 & 30.0 \\
(64, 1, 32, 256) & 4.9 & 65.0 & 20.2 & 35.0 & -0.1 & 4.9 & 45.0 & 35.0 & \textbf{75.0} & 65.0 & 65.0 \\
(64, 1, 64, 128) & 4.9 & 65.0 & 35.0 & 25.0 & -0.1 & 20.0 & 9.9 & 35.0 & \textbf{80.0} & 60.0 & 45.0 \\
(64, 1, 64, 256) & 4.9 & 65.0 & 35.0 & 35.0 & -0.1 & 20.0 & 45.0 & 35.0 & \textbf{75.0} & 65.0 & 70.0 \\
(64, 1, 128, 128) & 4.9 & 65.0 & 75.0 & 25.0 & -0.1 & 30.0 & 9.9 & 50.0 & \textbf{80.0} & \textbf{80.0} & 55.0 \\
(64, 1, 128, 256) & 4.9 & 65.0 & 75.0 & 35.0 & -0.1 & 30.0 & 45.0 & 50.0 & 75.0 & \textbf{85.0} & \textbf{85.0} \\
(64, 2, 32, 128) & 4.9 & 45.5 & 20.2 & 25.0 & -0.1 & 4.9 & 9.9 & 9.9 & \textbf{70.2} & 40.0 & 25.0 \\
(64, 2, 32, 256) & 4.9 & 45.5 & 20.2 & 35.0 & -0.1 & 4.9 & 45.0 & 9.9 & \textbf{85.0} & 65.0 & 60.0 \\
(64, 2, 64, 128) & 4.9 & 45.5 & 35.0 & 25.0 & -0.1 & 20.0 & 9.9 & 30.5 & \textbf{70.2} & 60.0 & 40.0 \\
(64, 2, 64, 256) & 4.9 & 45.5 & 35.0 & 35.0 & -0.1 & 20.0 & 45.0 & 30.5 & \textbf{85.0} & 65.0 & 75.0 \\
(64, 2, 128, 128) & 4.9 & 45.5 & 75.0 & 25.0 & -0.1 & 30.0 & 9.9 & 45.2 & 70.2 & \textbf{80.0} & 55.0 \\
(64, 2, 128, 256) & 4.9 & 45.5 & 75.0 & 35.0 & -0.1 & 30.0 & 45.0 & 45.2 & \textbf{85.0} & \textbf{85.0} & 80.0 \\
(128, 1, 32, 128) & 15.0 & 65.0 & 20.2 & 25.0 & 15.0 & 30.0 & 35.0 & 35.0 & \textbf{80.0} & 40.0 & 40.0 \\
(128, 1, 32, 256) & 15.0 & 65.0 & 20.2 & 35.0 & 15.0 & 30.0 & 50.0 & 35.0 & \textbf{75.0} & 65.0 & 60.0 \\
(128, 1, 64, 128) & 15.0 & 65.0 & 35.0 & 25.0 & 15.0 & 35.0 & 35.0 & 35.0 & \textbf{80.0} & 60.0 & 40.0 \\
(128, 1, 64, 256) & 15.0 & 65.0 & 35.0 & 35.0 & 15.0 & 35.0 & 50.0 & 35.0 & \textbf{75.0} & 65.0 & 60.0 \\
(128, 1, 128, 128) & 15.0 & 65.0 & 75.0 & 25.0 & 15.0 & 45.0 & 35.0 & 50.0 & \textbf{80.0} & \textbf{80.0} & 60.0 \\
(128, 1, 128, 256) & 15.0 & 65.0 & 75.0 & 35.0 & 15.0 & 45.0 & 50.0 & 50.0 & 75.0 & \textbf{85.0} & 70.0 \\
(128, 2, 32, 128) & 15.0 & 45.5 & 20.2 & 25.0 & 9.9 & 30.0 & 35.0 & 9.9 & \textbf{70.2} & 40.0 & 35.0 \\
(128, 2, 32, 256) & 15.0 & 45.5 & 20.2 & 35.0 & 9.9 & 30.0 & 50.0 & 9.9 & \textbf{85.0} & 65.0 & 55.0 \\
(128, 2, 64, 128) & 15.0 & 45.5 & 35.0 & 25.0 & 9.9 & 35.0 & 35.0 & 30.5 & \textbf{70.2} & 60.0 & 40.0 \\
(128, 2, 64, 256) & 15.0 & 45.5 & 35.0 & 35.0 & 9.9 & 35.0 & 50.0 & 30.5 & \textbf{85.0} & 65.0 & 60.0 \\
(128, 2, 128, 128) & 15.0 & 45.5 & 75.0 & 25.0 & 9.9 & 45.0 & 35.0 & 45.2 & 70.2 & \textbf{80.0} & 60.0 \\
(128, 2, 128, 256) & 15.0 & 45.5 & 75.0 & 35.0 & 9.9 & 45.0 & 50.0 & 45.2 & \textbf{85.0} & \textbf{85.0} & 75.0 \\
(256, 1, 32, 128) & 40.0 & 65.0 & 20.2 & 25.0 & 35.0 & 45.0 & 40.0 & 35.0 & \textbf{80.0} & 40.0 & 60.0 \\
(256, 1, 32, 256) & 40.0 & 65.0 & 20.2 & 35.0 & 35.0 & 45.0 & 60.0 & 35.0 & \textbf{75.0} & 65.0 & \textbf{75.0} \\
(256, 1, 64, 128) & 40.0 & 65.0 & 35.0 & 25.0 & 35.0 & 47.3 & 40.0 & 35.0 & \textbf{80.0} & 60.0 & 65.0 \\
(256, 1, 64, 256) & 40.0 & 65.0 & 35.0 & 35.0 & 35.0 & 47.3 & 60.0 & 35.0 & \textbf{75.0} & 65.0 & 70.0 \\
(256, 1, 128, 128) & 40.0 & 65.0 & 75.0 & 25.0 & 35.0 & 50.0 & 40.0 & 50.0 & \textbf{80.0} & \textbf{80.0} & 70.0 \\
(256, 1, 128, 256) & 40.0 & 65.0 & 75.0 & 35.0 & 35.0 & 50.0 & 60.0 & 50.0 & 75.0 & \textbf{85.0} & 75.0 \\
(256, 2, 32, 128) & 40.0 & 45.5 & 20.2 & 25.0 & 40.0 & 45.0 & 40.0 & 9.9 & \textbf{70.2} & 40.0 & 60.0 \\
(256, 2, 32, 256) & 40.0 & 45.5 & 20.2 & 35.0 & 40.0 & 45.0 & 60.0 & 9.9 & \textbf{85.0} & 65.0 & 65.0 \\
(256, 2, 64, 128) & 40.0 & 45.5 & 35.0 & 25.0 & 40.0 & 47.3 & 40.0 & 30.5 & \textbf{70.2} & 60.0 & 60.0 \\
(256, 2, 64, 256) & 40.0 & 45.5 & 35.0 & 35.0 & 40.0 & 47.3 & 60.0 & 30.5 & \textbf{85.0} & 65.0 & 70.0 \\
(256, 2, 128, 128) & 40.0 & 45.5 & 75.0 & 25.0 & 40.0 & 50.0 & 40.0 & 45.2 & 70.2 & \textbf{80.0} & 70.0 \\
(256, 2, 128, 256) & 40.0 & 45.5 & 75.0 & 35.0 & 40.0 & 50.0 & 60.0 & 45.2 & \textbf{85.0} & \textbf{85.0} & 80.0 \\
\bottomrule
\end{tabular}
\end{table}
% Requires: \usepackage{booktabs}
\begin{table}[htbp]
\centering
\small
\caption{Full results for Grid Trap (normalized discounted value, higher is better)}
\label{tab:appendix_grid_trap}
\begin{tabular}{lrrrr|rrrrrr|r}
\toprule
 & \multicolumn{4}{c|}{Singles} & \multicolumn{6}{c|}{Pairs} & \multicolumn{1}{c}{All} \\
Budget (P,D,R,S) & \fbPref & \fbDemo & \fbRating & \fbStop & \fbDemoPref & \fbPrefRating & \fbPrefStop & \fbDemoRating & \fbDemoStop & \fbRatingStop & \fbPDRS \\
\midrule
(64, 1, 32, 128) & 49.7 & 15.6 & 55.3 & -15.2 & 47.1 & 59.2 & 48.9 & 62.3 & \textbf{72.9} & 29.1 & 59.9 \\
(64, 1, 32, 256) & 49.7 & 15.6 & 55.3 & 56.1 & 47.1 & 59.2 & 64.1 & 62.3 & \textbf{69.6} & 67.6 & 64.9 \\
(64, 1, 64, 128) & 49.7 & 15.6 & 60.5 & -15.2 & 47.1 & \textbf{74.2} & 48.9 & 58.3 & 72.9 & 69.0 & 67.1 \\
(64, 1, 64, 256) & 49.7 & 15.6 & 60.5 & 56.1 & 47.1 & 74.2 & 64.1 & 58.3 & 69.6 & 76.2 & \textbf{83.1} \\
(64, 1, 128, 128) & 49.7 & 15.6 & \textbf{91.9} & -15.2 & 47.1 & 81.1 & 48.9 & 79.1 & 72.9 & 78.2 & 82.3 \\
(64, 1, 128, 256) & 49.7 & 15.6 & \textbf{91.9} & 56.1 & 47.1 & 81.1 & 64.1 & 79.1 & 69.6 & 82.5 & 89.2 \\
(64, 2, 32, 128) & 49.7 & 12.6 & 55.3 & -15.2 & 46.1 & 59.2 & 48.9 & 0.9 & 51.4 & 29.1 & \textbf{62.2} \\
(64, 2, 32, 256) & 49.7 & 12.6 & 55.3 & 56.1 & 46.1 & 59.2 & 64.1 & 0.9 & \textbf{73.6} & 67.6 & 66.8 \\
(64, 2, 64, 128) & 49.7 & 12.6 & 60.5 & -15.2 & 46.1 & \textbf{74.2} & 48.9 & 38.7 & 51.4 & 69.0 & 64.1 \\
(64, 2, 64, 256) & 49.7 & 12.6 & 60.5 & 56.1 & 46.1 & 74.2 & 64.1 & 38.7 & 73.6 & 76.2 & \textbf{77.6} \\
(64, 2, 128, 128) & 49.7 & 12.6 & \textbf{91.9} & -15.2 & 46.1 & 81.1 & 48.9 & 72.2 & 51.4 & 78.2 & 72.2 \\
(64, 2, 128, 256) & 49.7 & 12.6 & \textbf{91.9} & 56.1 & 46.1 & 81.1 & 64.1 & 72.2 & 73.6 & 82.5 & 86.5 \\
(128, 1, 32, 128) & 72.2 & 15.6 & 55.3 & -15.2 & 59.5 & \textbf{78.4} & 62.2 & 62.3 & 72.9 & 29.1 & 67.6 \\
(128, 1, 32, 256) & 72.2 & 15.6 & 55.3 & 56.1 & 59.5 & 78.4 & 78.4 & 62.3 & 69.6 & 67.6 & \textbf{86.7} \\
(128, 1, 64, 128) & 72.2 & 15.6 & 60.5 & -15.2 & 59.5 & \textbf{81.1} & 62.2 & 58.3 & 72.9 & 69.0 & 77.6 \\
(128, 1, 64, 256) & 72.2 & 15.6 & 60.5 & 56.1 & 59.5 & 81.1 & 78.4 & 58.3 & 69.6 & 76.2 & \textbf{86.5} \\
(128, 1, 128, 128) & 72.2 & 15.6 & \textbf{91.9} & -15.2 & 59.5 & 83.8 & 62.2 & 79.1 & 72.9 & 78.2 & 81.1 \\
(128, 1, 128, 256) & 72.2 & 15.6 & \textbf{91.9} & 56.1 & 59.5 & 83.8 & 78.4 & 79.1 & 69.6 & 82.5 & 86.5 \\
(128, 2, 32, 128) & 72.2 & 12.6 & 55.3 & -15.2 & 46.1 & \textbf{78.4} & 62.2 & 0.9 & 51.4 & 29.1 & 67.6 \\
(128, 2, 32, 256) & 72.2 & 12.6 & 55.3 & 56.1 & 46.1 & 78.4 & 78.4 & 0.9 & 73.6 & 67.6 & \textbf{83.8} \\
(128, 2, 64, 128) & 72.2 & 12.6 & 60.5 & -15.2 & 46.1 & \textbf{81.1} & 62.2 & 38.7 & 51.4 & 69.0 & 73.0 \\
(128, 2, 64, 256) & 72.2 & 12.6 & 60.5 & 56.1 & 46.1 & 81.1 & 78.4 & 38.7 & 73.6 & 76.2 & \textbf{86.5} \\
(128, 2, 128, 128) & 72.2 & 12.6 & \textbf{91.9} & -15.2 & 46.1 & 83.8 & 62.2 & 72.2 & 51.4 & 78.2 & 83.8 \\
(128, 2, 128, 256) & 72.2 & 12.6 & \textbf{91.9} & 56.1 & 46.1 & 83.8 & 78.4 & 72.2 & 73.6 & 82.5 & 86.5 \\
(256, 1, 32, 128) & 75.7 & 15.6 & 55.3 & -15.2 & 70.3 & \textbf{78.4} & 75.7 & 62.3 & 72.9 & 29.1 & 73.0 \\
(256, 1, 32, 256) & 75.7 & 15.6 & 55.3 & 56.1 & 70.3 & 78.4 & 75.9 & 62.3 & 69.6 & 67.6 & \textbf{81.1} \\
(256, 1, 64, 128) & 75.7 & 15.6 & 60.5 & -15.2 & 70.3 & \textbf{81.1} & 75.7 & 58.3 & 72.9 & 69.0 & 78.4 \\
(256, 1, 64, 256) & 75.7 & 15.6 & 60.5 & 56.1 & 70.3 & \textbf{81.1} & 75.9 & 58.3 & 69.6 & 76.2 & \textbf{81.1} \\
(256, 1, 128, 128) & 75.7 & 15.6 & \textbf{91.9} & -15.2 & 70.3 & 81.1 & 75.7 & 79.1 & 72.9 & 78.2 & 83.8 \\
(256, 1, 128, 256) & 75.7 & 15.6 & \textbf{91.9} & 56.1 & 70.3 & 81.1 & 75.9 & 79.1 & 69.6 & 82.5 & 86.5 \\
(256, 2, 32, 128) & 75.7 & 12.6 & 55.3 & -15.2 & 67.6 & \textbf{78.4} & 75.7 & 0.9 & 51.4 & 29.1 & 73.0 \\
(256, 2, 32, 256) & 75.7 & 12.6 & 55.3 & 56.1 & 67.6 & 78.4 & 75.9 & 0.9 & 73.6 & 67.6 & \textbf{81.1} \\
(256, 2, 64, 128) & 75.7 & 12.6 & 60.5 & -15.2 & 67.6 & \textbf{81.1} & 75.7 & 38.7 & 51.4 & 69.0 & 73.0 \\
(256, 2, 64, 256) & 75.7 & 12.6 & 60.5 & 56.1 & 67.6 & \textbf{81.1} & 75.9 & 38.7 & 73.6 & 76.2 & 78.4 \\
(256, 2, 128, 128) & 75.7 & 12.6 & \textbf{91.9} & -15.2 & 67.6 & 81.1 & 75.7 & 72.2 & 51.4 & 78.2 & 83.8 \\
(256, 2, 128, 256) & 75.7 & 12.6 & \textbf{91.9} & 56.1 & 67.6 & 81.1 & 75.9 & 72.2 & 73.6 & 82.5 & 89.3 \\
\bottomrule
\end{tabular}
\end{table}
% Requires: \usepackage{booktabs}
\begin{table}[htbp]
\centering
\small
\caption{Full results for Acrobot (v1) (normalized return, higher is better)}
\label{tab:appendix_acrobot_v1}
\begin{tabular}{lrrrr|rrrrrr|r}
\toprule
 & \multicolumn{4}{c|}{Singles} & \multicolumn{6}{c|}{Pairs} & \multicolumn{1}{c}{All} \\
Budget (P,D,R,S) & \fbPref & \fbDemo & \fbRating & \fbStop & \fbDemoPref & \fbPrefRating & \fbPrefStop & \fbDemoRating & \fbDemoStop & \fbRatingStop & \fbPDRS \\
\midrule
(256, 1, 32, 64) & 53.3 & 96.6 & 97.9 & 87.6 & 95.5 & 74.8 & 83.0 & 98.1 & \textbf{98.8} & 98.3 & 96.4 \\
(256, 1, 32, 128) & 53.3 & 96.6 & 97.9 & \textbf{99.1} & 95.5 & 74.8 & 93.2 & 98.1 & 98.8 & 98.5 & 98.7 \\
(256, 1, 64, 64) & 53.3 & 96.6 & 98.2 & 87.6 & 95.5 & 76.6 & 83.0 & \textbf{99.0} & 98.8 & 97.4 & 98.1 \\
(256, 1, 64, 128) & 53.3 & 96.6 & 98.2 & 99.1 & 95.5 & 76.6 & 93.2 & 99.0 & 98.8 & \textbf{99.3} & 98.6 \\
(256, 1, 128, 64) & 53.3 & 96.6 & 98.6 & 87.6 & 95.5 & 76.1 & 83.0 & 98.7 & 98.8 & 98.8 & \textbf{98.9} \\
(256, 1, 128, 128) & 53.3 & 96.6 & 98.6 & 99.1 & 95.5 & 76.1 & 93.2 & 98.7 & 98.8 & \textbf{99.2} & 98.5 \\
(256, 2, 32, 64) & 53.3 & 98.2 & 97.9 & 87.6 & 98.0 & 74.8 & 83.0 & 97.9 & \textbf{98.7} & 98.3 & 98.7 \\
(256, 2, 32, 128) & 53.3 & 98.2 & 97.9 & 99.1 & 98.0 & 74.8 & 93.2 & 97.9 & \textbf{99.1} & 98.5 & 98.5 \\
(256, 2, 64, 64) & 53.3 & 98.2 & 98.2 & 87.6 & 98.0 & 76.6 & 83.0 & \textbf{98.9} & 98.7 & 97.4 & 98.3 \\
(256, 2, 64, 128) & 53.3 & 98.2 & 98.2 & 99.1 & 98.0 & 76.6 & 93.2 & 98.9 & 99.1 & \textbf{99.3} & 98.6 \\
(256, 2, 128, 64) & 53.3 & 98.2 & 98.6 & 87.6 & 98.0 & 76.1 & 83.0 & 98.8 & 98.7 & \textbf{98.8} & 98.0 \\
(256, 2, 128, 128) & 53.3 & 98.2 & 98.6 & 99.1 & 98.0 & 76.1 & 93.2 & 98.8 & 99.1 & \textbf{99.2} & 99.1 \\
(256, 4, 32, 64) & 53.3 & \textbf{99.5} & 97.9 & 87.6 & 96.3 & 74.8 & 83.0 & 98.0 & 97.3 & 98.3 & 98.4 \\
(256, 4, 32, 128) & 53.3 & \textbf{99.5} & 97.9 & 99.1 & 96.3 & 74.8 & 93.2 & 98.0 & 98.9 & 98.5 & 99.1 \\
(256, 4, 64, 64) & 53.3 & \textbf{99.5} & 98.2 & 87.6 & 96.3 & 76.6 & 83.0 & 99.4 & 97.3 & 97.4 & 98.9 \\
(256, 4, 64, 128) & 53.3 & \textbf{99.5} & 98.2 & 99.1 & 96.3 & 76.6 & 93.2 & 99.4 & 98.9 & 99.3 & 98.6 \\
(256, 4, 128, 64) & 53.3 & \textbf{99.5} & 98.6 & 87.6 & 96.3 & 76.1 & 83.0 & 99.0 & 97.3 & 98.8 & 98.9 \\
(256, 4, 128, 128) & 53.3 & \textbf{99.5} & 98.6 & 99.1 & 96.3 & 76.1 & 93.2 & 99.0 & 98.9 & 99.2 & 98.8 \\
(256, 4, 256, 64) & 53.3 & \textbf{99.5} & 97.9 & 87.6 & 96.3 & 96.3 & 83.0 & 99.3 & 97.3 & 99.0 & 98.8 \\
(256, 4, 256, 128) & 53.3 & \textbf{99.5} & 97.9 & 99.1 & 96.3 & 96.3 & 93.2 & 99.3 & 98.9 & 99.2 & 99.0 \\
(256, 4, 512, 64) & 53.3 & \textbf{99.5} & 73.4 & 87.6 & 96.3 & 70.7 & 83.0 & 99.2 & 97.3 & 98.1 & 99.1 \\
(256, 4, 512, 128) & 53.3 & \textbf{99.5} & 73.4 & 99.1 & 96.3 & 70.7 & 93.2 & 99.2 & 98.9 & 99.5 & 99.4 \\
(512, 1, 32, 64) & 53.3 & 96.6 & 97.9 & 87.6 & 94.3 & 60.6 & 96.6 & 98.1 & \textbf{98.8} & 98.3 & 97.6 \\
(512, 1, 32, 128) & 53.3 & 96.6 & 97.9 & \textbf{99.1} & 94.3 & 60.6 & 79.8 & 98.1 & 98.8 & 98.5 & 98.6 \\
(512, 1, 64, 64) & 53.3 & 96.6 & 98.2 & 87.6 & 94.3 & 84.8 & 96.6 & \textbf{99.0} & 98.8 & 97.4 & 98.5 \\
(512, 1, 64, 128) & 53.3 & 96.6 & 98.2 & 99.1 & 94.3 & 84.8 & 79.8 & 99.0 & 98.8 & \textbf{99.3} & 98.4 \\
(512, 1, 128, 64) & 53.3 & 96.6 & 98.6 & 87.6 & 94.3 & 78.4 & 96.6 & 98.7 & 98.8 & \textbf{98.8} & 98.6 \\
(512, 1, 128, 128) & 53.3 & 96.6 & 98.6 & 99.1 & 94.3 & 78.4 & 79.8 & 98.7 & 98.8 & \textbf{99.2} & 98.8 \\
(512, 2, 32, 64) & 53.3 & 98.2 & 97.9 & 87.6 & 97.4 & 60.6 & 96.6 & 97.9 & \textbf{98.7} & 98.3 & 98.4 \\
(512, 2, 32, 128) & 53.3 & 98.2 & 97.9 & 99.1 & 97.4 & 60.6 & 79.8 & 97.9 & \textbf{99.1} & 98.5 & 98.2 \\
(512, 2, 64, 64) & 53.3 & 98.2 & 98.2 & 87.6 & 97.4 & 84.8 & 96.6 & \textbf{98.9} & 98.7 & 97.4 & 98.6 \\
(512, 2, 64, 128) & 53.3 & 98.2 & 98.2 & 99.1 & 97.4 & 84.8 & 79.8 & 98.9 & 99.1 & \textbf{99.3} & 98.4 \\
(512, 2, 128, 64) & 53.3 & 98.2 & 98.6 & 87.6 & 97.4 & 78.4 & 96.6 & 98.8 & 98.7 & 98.8 & \textbf{98.9} \\
(512, 2, 128, 128) & 53.3 & 98.2 & 98.6 & 99.1 & 97.4 & 78.4 & 79.8 & 98.8 & 99.1 & \textbf{99.2} & 99.1 \\
(512, 4, 32, 64) & 53.3 & \textbf{99.5} & 97.9 & 87.6 & 98.3 & 60.6 & 96.6 & 98.0 & 97.3 & 98.3 & 99.2 \\
(512, 4, 32, 128) & 53.3 & \textbf{99.5} & 97.9 & 99.1 & 98.3 & 60.6 & 79.8 & 98.0 & 98.9 & 98.5 & 99.0 \\
(512, 4, 64, 64) & 53.3 & \textbf{99.5} & 98.2 & 87.6 & 98.3 & 84.8 & 96.6 & 99.4 & 97.3 & 97.4 & 99.2 \\
(512, 4, 64, 128) & 53.3 & \textbf{99.5} & 98.2 & 99.1 & 98.3 & 84.8 & 79.8 & 99.4 & 98.9 & 99.3 & 99.1 \\
(512, 4, 128, 64) & 53.3 & \textbf{99.5} & 98.6 & 87.6 & 98.3 & 78.4 & 96.6 & 99.0 & 97.3 & 98.8 & 98.8 \\
(512, 4, 128, 128) & 53.3 & \textbf{99.5} & 98.6 & 99.1 & 98.3 & 78.4 & 79.8 & 99.0 & 98.9 & 99.2 & 99.2 \\
(512, 4, 256, 64) & 53.3 & \textbf{99.5} & 97.9 & 87.6 & 98.3 & 88.8 & 96.6 & 99.3 & 97.3 & 99.0 & 99.0 \\
(512, 4, 256, 128) & 53.3 & \textbf{99.5} & 97.9 & 99.1 & 98.3 & 88.8 & 79.8 & 99.3 & 98.9 & 99.2 & 99.2 \\
(512, 4, 512, 64) & 53.3 & \textbf{99.5} & 73.4 & 87.6 & 98.3 & 97.3 & 96.6 & 99.2 & 97.3 & 98.1 & 99.1 \\
(512, 4, 512, 128) & 53.3 & \textbf{99.5} & 73.4 & 99.1 & 98.3 & 97.3 & 79.8 & 99.2 & 98.9 & 99.5 & 99.1 \\
\bottomrule
\end{tabular}
\end{table}
% Requires: \usepackage{booktabs}
\begin{table}[htbp]
\centering
\small
\caption{Full results for CartPole (v1) (normalized return, higher is better)}
\label{tab:appendix_cartpole_v1}
\begin{tabular}{lrrrr|rrrrrr|r}
\toprule
 & \multicolumn{4}{c|}{Singles} & \multicolumn{6}{c|}{Pairs} & \multicolumn{1}{c}{All} \\
Budget (P,D,R,S) & \fbPref & \fbDemo & \fbRating & \fbStop & \fbDemoPref & \fbPrefRating & \fbPrefStop & \fbDemoRating & \fbDemoStop & \fbRatingStop & \fbPDRS \\
\midrule
(256, 1, 32, 64) & 64.7 & 24.2 & \textbf{81.4} & -1.3 & 50.8 & 71.5 & 51.1 & 32.7 & -1.0 & 33.3 & 37.3 \\
(256, 1, 32, 128) & 64.7 & 24.2 & \textbf{81.4} & 1.0 & 50.8 & 71.5 & 44.1 & 32.7 & -1.4 & 27.4 & 26.9 \\
(256, 1, 64, 64) & 64.7 & 24.2 & 78.5 & -1.3 & 50.8 & \textbf{82.3} & 51.1 & 45.0 & -1.0 & 51.8 & 32.9 \\
(256, 1, 64, 128) & 64.7 & 24.2 & 78.5 & 1.0 & 50.8 & \textbf{82.3} & 44.1 & 45.0 & -1.4 & 58.7 & 27.4 \\
(256, 1, 128, 64) & 64.7 & 24.2 & 73.8 & -1.3 & 50.8 & \textbf{92.5} & 51.1 & 59.3 & -1.0 & 74.7 & 62.3 \\
(256, 1, 128, 128) & 64.7 & 24.2 & 73.8 & 1.0 & 50.8 & \textbf{92.5} & 44.1 & 59.3 & -1.4 & 57.4 & 46.2 \\
(256, 2, 32, 64) & 64.7 & 38.4 & \textbf{81.4} & -1.3 & 62.9 & 71.5 & 51.1 & 38.1 & 4.8 & 33.3 & 48.4 \\
(256, 2, 32, 128) & 64.7 & 38.4 & \textbf{81.4} & 1.0 & 62.9 & 71.5 & 44.1 & 38.1 & -1.3 & 27.4 & 24.9 \\
(256, 2, 64, 64) & 64.7 & 38.4 & 78.5 & -1.3 & 62.9 & \textbf{82.3} & 51.1 & 37.2 & 4.8 & 51.8 & 42.5 \\
(256, 2, 64, 128) & 64.7 & 38.4 & 78.5 & 1.0 & 62.9 & \textbf{82.3} & 44.1 & 37.2 & -1.3 & 58.7 & 34.5 \\
(256, 2, 128, 64) & 64.7 & 38.4 & 73.8 & -1.3 & 62.9 & \textbf{92.5} & 51.1 & 62.3 & 4.8 & 74.7 & 57.2 \\
(256, 2, 128, 128) & 64.7 & 38.4 & 73.8 & 1.0 & 62.9 & \textbf{92.5} & 44.1 & 62.3 & -1.3 & 57.4 & 37.7 \\
(256, 4, 32, 64) & 64.7 & 26.5 & \textbf{81.4} & -1.3 & 66.1 & 71.5 & 51.1 & 40.8 & 12.2 & 33.3 & 29.6 \\
(256, 4, 32, 128) & 64.7 & 26.5 & \textbf{81.4} & 1.0 & 66.1 & 71.5 & 44.1 & 40.8 & 1.7 & 27.4 & 23.1 \\
(256, 4, 64, 64) & 64.7 & 26.5 & 78.5 & -1.3 & 66.1 & \textbf{82.3} & 51.1 & 46.2 & 12.2 & 51.8 & 41.6 \\
(256, 4, 64, 128) & 64.7 & 26.5 & 78.5 & 1.0 & 66.1 & \textbf{82.3} & 44.1 & 46.2 & 1.7 & 58.7 & 51.5 \\
(256, 4, 128, 64) & 64.7 & 26.5 & 73.8 & -1.3 & 66.1 & \textbf{92.5} & 51.1 & 72.7 & 12.2 & 74.7 & 61.7 \\
(256, 4, 128, 128) & 64.7 & 26.5 & 73.8 & 1.0 & 66.1 & \textbf{92.5} & 44.1 & 72.7 & 1.7 & 57.4 & 50.9 \\
(256, 4, 256, 64) & 64.7 & 26.5 & 69.8 & -1.3 & 66.1 & \textbf{97.7} & 51.1 & 62.5 & 12.2 & 93.8 & 87.5 \\
(256, 4, 256, 128) & 64.7 & 26.5 & 69.8 & 1.0 & 66.1 & \textbf{97.7} & 44.1 & 62.5 & 1.7 & 70.5 & 72.3 \\
(256, 4, 512, 64) & 64.7 & 26.5 & \textbf{96.4} & -1.3 & 66.1 & 96.2 & 51.1 & 87.7 & 12.2 & 93.4 & 81.9 \\
(256, 4, 512, 128) & 64.7 & 26.5 & 96.4 & 1.0 & 66.1 & 96.2 & 44.1 & 87.7 & 1.7 & \textbf{98.4} & 86.7 \\
(512, 1, 32, 64) & 67.1 & 24.2 & 81.4 & -1.3 & 66.8 & \textbf{94.7} & 43.7 & 32.7 & -1.0 & 33.3 & 43.3 \\
(512, 1, 32, 128) & 67.1 & 24.2 & 81.4 & 1.0 & 66.8 & \textbf{94.7} & 50.4 & 32.7 & -1.4 & 27.4 & 34.0 \\
(512, 1, 64, 64) & 67.1 & 24.2 & 78.5 & -1.3 & 66.8 & \textbf{88.7} & 43.7 & 45.0 & -1.0 & 51.8 & 50.0 \\
(512, 1, 64, 128) & 67.1 & 24.2 & 78.5 & 1.0 & 66.8 & \textbf{88.7} & 50.4 & 45.0 & -1.4 & 58.7 & 31.1 \\
(512, 1, 128, 64) & 67.1 & 24.2 & 73.8 & -1.3 & 66.8 & \textbf{99.9} & 43.7 & 59.3 & -1.0 & 74.7 & 53.7 \\
(512, 1, 128, 128) & 67.1 & 24.2 & 73.8 & 1.0 & 66.8 & \textbf{99.9} & 50.4 & 59.3 & -1.4 & 57.4 & 42.8 \\
(512, 2, 32, 64) & 67.1 & 38.4 & 81.4 & -1.3 & 83.4 & \textbf{94.7} & 43.7 & 38.1 & 4.8 & 33.3 & 44.6 \\
(512, 2, 32, 128) & 67.1 & 38.4 & 81.4 & 1.0 & 83.4 & \textbf{94.7} & 50.4 & 38.1 & -1.3 & 27.4 & 41.2 \\
(512, 2, 64, 64) & 67.1 & 38.4 & 78.5 & -1.3 & 83.4 & \textbf{88.7} & 43.7 & 37.2 & 4.8 & 51.8 & 55.8 \\
(512, 2, 64, 128) & 67.1 & 38.4 & 78.5 & 1.0 & 83.4 & \textbf{88.7} & 50.4 & 37.2 & -1.3 & 58.7 & 42.5 \\
(512, 2, 128, 64) & 67.1 & 38.4 & 73.8 & -1.3 & 83.4 & \textbf{99.9} & 43.7 & 62.3 & 4.8 & 74.7 & 67.6 \\
(512, 2, 128, 128) & 67.1 & 38.4 & 73.8 & 1.0 & 83.4 & \textbf{99.9} & 50.4 & 62.3 & -1.3 & 57.4 & 48.8 \\
(512, 4, 32, 64) & 67.1 & 26.5 & 81.4 & -1.3 & 78.6 & \textbf{94.7} & 43.7 & 40.8 & 12.2 & 33.3 & 41.3 \\
(512, 4, 32, 128) & 67.1 & 26.5 & 81.4 & 1.0 & 78.6 & \textbf{94.7} & 50.4 & 40.8 & 1.7 & 27.4 & 29.6 \\
(512, 4, 64, 64) & 67.1 & 26.5 & 78.5 & -1.3 & 78.6 & \textbf{88.7} & 43.7 & 46.2 & 12.2 & 51.8 & 47.7 \\
(512, 4, 64, 128) & 67.1 & 26.5 & 78.5 & 1.0 & 78.6 & \textbf{88.7} & 50.4 & 46.2 & 1.7 & 58.7 & 30.5 \\
(512, 4, 128, 64) & 67.1 & 26.5 & 73.8 & -1.3 & 78.6 & \textbf{99.9} & 43.7 & 72.7 & 12.2 & 74.7 & 48.4 \\
(512, 4, 128, 128) & 67.1 & 26.5 & 73.8 & 1.0 & 78.6 & \textbf{99.9} & 50.4 & 72.7 & 1.7 & 57.4 & 47.6 \\
(512, 4, 256, 64) & 67.1 & 26.5 & 69.8 & -1.3 & 78.6 & \textbf{100.0} & 43.7 & 62.5 & 12.2 & 93.8 & 88.1 \\
(512, 4, 256, 128) & 67.1 & 26.5 & 69.8 & 1.0 & 78.6 & \textbf{100.0} & 50.4 & 62.5 & 1.7 & 70.5 & 52.0 \\
(512, 4, 512, 64) & 67.1 & 26.5 & 96.4 & -1.3 & 78.6 & \textbf{98.5} & 43.7 & 87.7 & 12.2 & 93.4 & 85.5 \\
(512, 4, 512, 128) & 67.1 & 26.5 & 96.4 & 1.0 & 78.6 & \textbf{98.5} & 50.4 & 87.7 & 1.7 & 98.4 & 85.8 \\
\bottomrule
\end{tabular}
\end{table}
% Requires: \usepackage{booktabs}
\begin{table}[htbp]
\centering
\small
\caption{Full results for LunarLander-v3 (normalized return, higher is better)}
\label{tab:appendix_lunarlander_v3}
\begin{tabular}{lrrrr|rrrrrr|r}
\toprule
 & \multicolumn{4}{c|}{Singles} & \multicolumn{6}{c|}{Pairs} & \multicolumn{1}{c}{All} \\
Budget (P,D,R,S) & \fbPref & \fbDemo & \fbRating & \fbStop & \fbDemoPref & \fbPrefRating & \fbPrefStop & \fbDemoRating & \fbDemoStop & \fbRatingStop & \fbPDRS \\
\midrule
(512, 1, 512, 128) & -15.8 & -0.2 & \textbf{23.7} & -30.3 & -3.7 & 11.7 & -15.9 & -38.4 & -59.1 & -11.0 & -2.1 \\
(512, 1, 512, 256) & -15.8 & -0.2 & \textbf{23.7} & -22.2 & -3.7 & 11.7 & 1.4 & -38.4 & -10.4 & 15.1 & 2.0 \\
(512, 1, 1024, 128) & -15.8 & -0.2 & 3.6 & -30.3 & -3.7 & -0.2 & -15.9 & -13.0 & -59.1 & \textbf{11.6} & 2.9 \\
(512, 1, 1024, 256) & -15.8 & -0.2 & 3.6 & -22.2 & -3.7 & -0.2 & 1.4 & -13.0 & -10.4 & \textbf{17.6} & 11.2 \\
(512, 2, 512, 128) & -15.8 & \textbf{108.9} & 23.7 & -30.3 & -12.8 & 11.7 & -15.9 & -16.2 & -25.3 & -11.0 & -7.5 \\
(512, 2, 512, 256) & -15.8 & \textbf{108.9} & 23.7 & -22.2 & -12.8 & 11.7 & 1.4 & -16.2 & -13.9 & 15.1 & 17.5 \\
(512, 2, 1024, 128) & -15.8 & \textbf{108.9} & 3.6 & -30.3 & -12.8 & -0.2 & -15.9 & -1.1 & -25.3 & 11.6 & 10.4 \\
(512, 2, 1024, 256) & -15.8 & \textbf{108.9} & 3.6 & -22.2 & -12.8 & -0.2 & 1.4 & -1.1 & -13.9 & 17.6 & 6.5 \\
(512, 4, 512, 128) & -15.8 & \textbf{113.7} & 23.7 & -30.3 & -29.0 & 11.7 & -15.9 & 8.2 & -34.5 & -11.0 & 12.2 \\
(512, 4, 512, 256) & -15.8 & \textbf{113.7} & 23.7 & -22.2 & -29.0 & 11.7 & 1.4 & 8.2 & 5.0 & 15.1 & 20.2 \\
(512, 4, 1024, 128) & -15.8 & \textbf{113.7} & 3.6 & -30.3 & -29.0 & -0.2 & -15.9 & 8.0 & -34.5 & 11.6 & 7.8 \\
(512, 4, 1024, 256) & -15.8 & \textbf{113.7} & 3.6 & -22.2 & -29.0 & -0.2 & 1.4 & 8.0 & 5.0 & 17.6 & 24.7 \\
(512, 32, 512, 128) & -15.8 & \textbf{115.6} & 23.7 & -30.3 & 39.3 & 11.7 & -15.9 & 42.7 & 39.3 & -11.0 & 59.7 \\
(512, 32, 512, 256) & -15.8 & \textbf{115.6} & 23.7 & -22.2 & 39.3 & 11.7 & 1.4 & 42.7 & 55.7 & 15.1 & 63.4 \\
(512, 32, 1024, 128) & -15.8 & \textbf{115.6} & 3.6 & -30.3 & 39.3 & -0.2 & -15.9 & 38.3 & 39.3 & 11.6 & 71.3 \\
(512, 32, 1024, 256) & -15.8 & \textbf{115.6} & 3.6 & -22.2 & 39.3 & -0.2 & 1.4 & 38.3 & 55.7 & 17.6 & 73.9 \\
(1024, 1, 512, 128) & -3.8 & -0.2 & \textbf{23.7} & -30.3 & 14.3 & -7.1 & -2.6 & -38.4 & -59.1 & -11.0 & 11.8 \\
(1024, 1, 512, 256) & -3.8 & -0.2 & \textbf{23.7} & -22.2 & 14.3 & -7.1 & 1.2 & -38.4 & -10.4 & 15.1 & 7.9 \\
(1024, 1, 1024, 128) & -3.8 & -0.2 & 3.6 & -30.3 & 14.3 & 4.0 & -2.6 & -13.0 & -59.1 & 11.6 & \textbf{16.3} \\
(1024, 1, 1024, 256) & -3.8 & -0.2 & 3.6 & -22.2 & 14.3 & 4.0 & 1.2 & -13.0 & -10.4 & \textbf{17.6} & 8.9 \\
(1024, 2, 512, 128) & -3.8 & \textbf{108.9} & 23.7 & -30.3 & 4.5 & -7.1 & -2.6 & -16.2 & -25.3 & -11.0 & -1.2 \\
(1024, 2, 512, 256) & -3.8 & \textbf{108.9} & 23.7 & -22.2 & 4.5 & -7.1 & 1.2 & -16.2 & -13.9 & 15.1 & 20.5 \\
(1024, 2, 1024, 128) & -3.8 & \textbf{108.9} & 3.6 & -30.3 & 4.5 & 4.0 & -2.6 & -1.1 & -25.3 & 11.6 & 8.5 \\
(1024, 2, 1024, 256) & -3.8 & \textbf{108.9} & 3.6 & -22.2 & 4.5 & 4.0 & 1.2 & -1.1 & -13.9 & 17.6 & -0.3 \\
(1024, 4, 512, 128) & -3.8 & \textbf{113.7} & 23.7 & -30.3 & 11.2 & -7.1 & -2.6 & 8.2 & -34.5 & -11.0 & 8.0 \\
(1024, 4, 512, 256) & -3.8 & \textbf{113.7} & 23.7 & -22.2 & 11.2 & -7.1 & 1.2 & 8.2 & 5.0 & 15.1 & 18.5 \\
(1024, 4, 1024, 128) & -3.8 & \textbf{113.7} & 3.6 & -30.3 & 11.2 & 4.0 & -2.6 & 8.0 & -34.5 & 11.6 & 22.6 \\
(1024, 4, 1024, 256) & -3.8 & \textbf{113.7} & 3.6 & -22.2 & 11.2 & 4.0 & 1.2 & 8.0 & 5.0 & 17.6 & 23.0 \\
(1024, 32, 512, 128) & -3.8 & \textbf{115.6} & 23.7 & -30.3 & 30.0 & -7.1 & -2.6 & 42.7 & 39.3 & -11.0 & 71.0 \\
(1024, 32, 512, 256) & -3.8 & \textbf{115.6} & 23.7 & -22.2 & 30.0 & -7.1 & 1.2 & 42.7 & 55.7 & 15.1 & 77.8 \\
(1024, 32, 1024, 128) & -3.8 & \textbf{115.6} & 3.6 & -30.3 & 30.0 & 4.0 & -2.6 & 38.3 & 39.3 & 11.6 & 67.2 \\
(1024, 32, 1024, 256) & -3.8 & \textbf{115.6} & 3.6 & -22.2 & 30.0 & 4.0 & 1.2 & 38.3 & 55.7 & 17.6 & 80.4 \\
\bottomrule
\end{tabular}
\end{table}
