# Supplementary material for: MAVRL: Learning Reward Functions from Multiple Feedback Types with Amortized Variational Inference
Source: arXiv:2602.15206 source file (2026-06-19)
Supplement: Supplementary file 2 [file table_appendix_acrobot_v1.tex]

% Requires: \usepackage{booktabs}
\begin{table}[htbp]
\centering
\small
\caption{Full results for Acrobot (v1) (normalized return, higher is better)}
\label{tab:appendix_acrobot_v1}
\begin{tabular}{lrrrr|rrrrrr|r}
\toprule
 & \multicolumn{4}{c|}{Singles} & \multicolumn{6}{c|}{Pairs} & \multicolumn{1}{c}{All} \\
Budget (P,D,R,S) & \fbPref & \fbDemo & \fbRating & \fbStop & \fbDemoPref & \fbPrefRating & \fbPrefStop & \fbDemoRating & \fbDemoStop & \fbRatingStop & \fbPDRS \\
\midrule
(256, 1, 32, 64) & 53.3 & 96.6 & 97.9 & 87.6 & 95.5 & 74.8 & 83.0 & 98.1 & \textbf{98.8} & 98.3 & 96.4 \\
(256, 1, 32, 128) & 53.3 & 96.6 & 97.9 & \textbf{99.1} & 95.5 & 74.8 & 93.2 & 98.1 & 98.8 & 98.5 & 98.7 \\
(256, 1, 64, 64) & 53.3 & 96.6 & 98.2 & 87.6 & 95.5 & 76.6 & 83.0 & \textbf{99.0} & 98.8 & 97.4 & 98.1 \\
(256, 1, 64, 128) & 53.3 & 96.6 & 98.2 & 99.1 & 95.5 & 76.6 & 93.2 & 99.0 & 98.8 & \textbf{99.3} & 98.6 \\
(256, 1, 128, 64) & 53.3 & 96.6 & 98.6 & 87.6 & 95.5 & 76.1 & 83.0 & 98.7 & 98.8 & 98.8 & \textbf{98.9} \\
(256, 1, 128, 128) & 53.3 & 96.6 & 98.6 & 99.1 & 95.5 & 76.1 & 93.2 & 98.7 & 98.8 & \textbf{99.2} & 98.5 \\
(256, 2, 32, 64) & 53.3 & 98.2 & 97.9 & 87.6 & 98.0 & 74.8 & 83.0 & 97.9 & \textbf{98.7} & 98.3 & 98.7 \\
(256, 2, 32, 128) & 53.3 & 98.2 & 97.9 & 99.1 & 98.0 & 74.8 & 93.2 & 97.9 & \textbf{99.1} & 98.5 & 98.5 \\
(256, 2, 64, 64) & 53.3 & 98.2 & 98.2 & 87.6 & 98.0 & 76.6 & 83.0 & \textbf{98.9} & 98.7 & 97.4 & 98.3 \\
(256, 2, 64, 128) & 53.3 & 98.2 & 98.2 & 99.1 & 98.0 & 76.6 & 93.2 & 98.9 & 99.1 & \textbf{99.3} & 98.6 \\
(256, 2, 128, 64) & 53.3 & 98.2 & 98.6 & 87.6 & 98.0 & 76.1 & 83.0 & 98.8 & 98.7 & \textbf{98.8} & 98.0 \\
(256, 2, 128, 128) & 53.3 & 98.2 & 98.6 & 99.1 & 98.0 & 76.1 & 93.2 & 98.8 & 99.1 & \textbf{99.2} & 99.1 \\
(256, 4, 32, 64) & 53.3 & \textbf{99.5} & 97.9 & 87.6 & 96.3 & 74.8 & 83.0 & 98.0 & 97.3 & 98.3 & 98.4 \\
(256, 4, 32, 128) & 53.3 & \textbf{99.5} & 97.9 & 99.1 & 96.3 & 74.8 & 93.2 & 98.0 & 98.9 & 98.5 & 99.1 \\
(256, 4, 64, 64) & 53.3 & \textbf{99.5} & 98.2 & 87.6 & 96.3 & 76.6 & 83.0 & 99.4 & 97.3 & 97.4 & 98.9 \\
(256, 4, 64, 128) & 53.3 & \textbf{99.5} & 98.2 & 99.1 & 96.3 & 76.6 & 93.2 & 99.4 & 98.9 & 99.3 & 98.6 \\
(256, 4, 128, 64) & 53.3 & \textbf{99.5} & 98.6 & 87.6 & 96.3 & 76.1 & 83.0 & 99.0 & 97.3 & 98.8 & 98.9 \\
(256, 4, 128, 128) & 53.3 & \textbf{99.5} & 98.6 & 99.1 & 96.3 & 76.1 & 93.2 & 99.0 & 98.9 & 99.2 & 98.8 \\
(256, 4, 256, 64) & 53.3 & \textbf{99.5} & 97.9 & 87.6 & 96.3 & 96.3 & 83.0 & 99.3 & 97.3 & 99.0 & 98.8 \\
(256, 4, 256, 128) & 53.3 & \textbf{99.5} & 97.9 & 99.1 & 96.3 & 96.3 & 93.2 & 99.3 & 98.9 & 99.2 & 99.0 \\
(256, 4, 512, 64) & 53.3 & \textbf{99.5} & 73.4 & 87.6 & 96.3 & 70.7 & 83.0 & 99.2 & 97.3 & 98.1 & 99.1 \\
(256, 4, 512, 128) & 53.3 & \textbf{99.5} & 73.4 & 99.1 & 96.3 & 70.7 & 93.2 & 99.2 & 98.9 & 99.5 & 99.4 \\
(512, 1, 32, 64) & 53.3 & 96.6 & 97.9 & 87.6 & 94.3 & 60.6 & 96.6 & 98.1 & \textbf{98.8} & 98.3 & 97.6 \\
(512, 1, 32, 128) & 53.3 & 96.6 & 97.9 & \textbf{99.1} & 94.3 & 60.6 & 79.8 & 98.1 & 98.8 & 98.5 & 98.6 \\
(512, 1, 64, 64) & 53.3 & 96.6 & 98.2 & 87.6 & 94.3 & 84.8 & 96.6 & \textbf{99.0} & 98.8 & 97.4 & 98.5 \\
(512, 1, 64, 128) & 53.3 & 96.6 & 98.2 & 99.1 & 94.3 & 84.8 & 79.8 & 99.0 & 98.8 & \textbf{99.3} & 98.4 \\
(512, 1, 128, 64) & 53.3 & 96.6 & 98.6 & 87.6 & 94.3 & 78.4 & 96.6 & 98.7 & 98.8 & \textbf{98.8} & 98.6 \\
(512, 1, 128, 128) & 53.3 & 96.6 & 98.6 & 99.1 & 94.3 & 78.4 & 79.8 & 98.7 & 98.8 & \textbf{99.2} & 98.8 \\
(512, 2, 32, 64) & 53.3 & 98.2 & 97.9 & 87.6 & 97.4 & 60.6 & 96.6 & 97.9 & \textbf{98.7} & 98.3 & 98.4 \\
(512, 2, 32, 128) & 53.3 & 98.2 & 97.9 & 99.1 & 97.4 & 60.6 & 79.8 & 97.9 & \textbf{99.1} & 98.5 & 98.2 \\
(512, 2, 64, 64) & 53.3 & 98.2 & 98.2 & 87.6 & 97.4 & 84.8 & 96.6 & \textbf{98.9} & 98.7 & 97.4 & 98.6 \\
(512, 2, 64, 128) & 53.3 & 98.2 & 98.2 & 99.1 & 97.4 & 84.8 & 79.8 & 98.9 & 99.1 & \textbf{99.3} & 98.4 \\
(512, 2, 128, 64) & 53.3 & 98.2 & 98.6 & 87.6 & 97.4 & 78.4 & 96.6 & 98.8 & 98.7 & 98.8 & \textbf{98.9} \\
(512, 2, 128, 128) & 53.3 & 98.2 & 98.6 & 99.1 & 97.4 & 78.4 & 79.8 & 98.8 & 99.1 & \textbf{99.2} & 99.1 \\
(512, 4, 32, 64) & 53.3 & \textbf{99.5} & 97.9 & 87.6 & 98.3 & 60.6 & 96.6 & 98.0 & 97.3 & 98.3 & 99.2 \\
(512, 4, 32, 128) & 53.3 & \textbf{99.5} & 97.9 & 99.1 & 98.3 & 60.6 & 79.8 & 98.0 & 98.9 & 98.5 & 99.0 \\
(512, 4, 64, 64) & 53.3 & \textbf{99.5} & 98.2 & 87.6 & 98.3 & 84.8 & 96.6 & 99.4 & 97.3 & 97.4 & 99.2 \\
(512, 4, 64, 128) & 53.3 & \textbf{99.5} & 98.2 & 99.1 & 98.3 & 84.8 & 79.8 & 99.4 & 98.9 & 99.3 & 99.1 \\
(512, 4, 128, 64) & 53.3 & \textbf{99.5} & 98.6 & 87.6 & 98.3 & 78.4 & 96.6 & 99.0 & 97.3 & 98.8 & 98.8 \\
(512, 4, 128, 128) & 53.3 & \textbf{99.5} & 98.6 & 99.1 & 98.3 & 78.4 & 79.8 & 99.0 & 98.9 & 99.2 & 99.2 \\
(512, 4, 256, 64) & 53.3 & \textbf{99.5} & 97.9 & 87.6 & 98.3 & 88.8 & 96.6 & 99.3 & 97.3 & 99.0 & 99.0 \\
(512, 4, 256, 128) & 53.3 & \textbf{99.5} & 97.9 & 99.1 & 98.3 & 88.8 & 79.8 & 99.3 & 98.9 & 99.2 & 99.2 \\
(512, 4, 512, 64) & 53.3 & \textbf{99.5} & 73.4 & 87.6 & 98.3 & 97.3 & 96.6 & 99.2 & 97.3 & 98.1 & 99.1 \\
(512, 4, 512, 128) & 53.3 & \textbf{99.5} & 73.4 & 99.1 & 98.3 & 97.3 & 79.8 & 99.2 & 98.9 & 99.5 & 99.1 \\
\bottomrule
\end{tabular}
\end{table}
