# Supplementary material for: MAVRL: Learning Reward Functions from Multiple Feedback Types with Amortized Variational Inference
Source: arXiv:2602.15206 source file (2026-06-19)
Supplement: Supplementary file 3 [file table_appendix_cartpole_v1.tex]

% Requires: \usepackage{booktabs}
\begin{table}[htbp]
\centering
\small
\caption{Full results for CartPole (v1) (normalized return, higher is better)}
\label{tab:appendix_cartpole_v1}
\begin{tabular}{lrrrr|rrrrrr|r}
\toprule
 & \multicolumn{4}{c|}{Singles} & \multicolumn{6}{c|}{Pairs} & \multicolumn{1}{c}{All} \\
Budget (P,D,R,S) & \fbPref & \fbDemo & \fbRating & \fbStop & \fbDemoPref & \fbPrefRating & \fbPrefStop & \fbDemoRating & \fbDemoStop & \fbRatingStop & \fbPDRS \\
\midrule
(256, 1, 32, 64) & 64.7 & 24.2 & \textbf{81.4} & -1.3 & 50.8 & 71.5 & 51.1 & 32.7 & -1.0 & 33.3 & 37.3 \\
(256, 1, 32, 128) & 64.7 & 24.2 & \textbf{81.4} & 1.0 & 50.8 & 71.5 & 44.1 & 32.7 & -1.4 & 27.4 & 26.9 \\
(256, 1, 64, 64) & 64.7 & 24.2 & 78.5 & -1.3 & 50.8 & \textbf{82.3} & 51.1 & 45.0 & -1.0 & 51.8 & 32.9 \\
(256, 1, 64, 128) & 64.7 & 24.2 & 78.5 & 1.0 & 50.8 & \textbf{82.3} & 44.1 & 45.0 & -1.4 & 58.7 & 27.4 \\
(256, 1, 128, 64) & 64.7 & 24.2 & 73.8 & -1.3 & 50.8 & \textbf{92.5} & 51.1 & 59.3 & -1.0 & 74.7 & 62.3 \\
(256, 1, 128, 128) & 64.7 & 24.2 & 73.8 & 1.0 & 50.8 & \textbf{92.5} & 44.1 & 59.3 & -1.4 & 57.4 & 46.2 \\
(256, 2, 32, 64) & 64.7 & 38.4 & \textbf{81.4} & -1.3 & 62.9 & 71.5 & 51.1 & 38.1 & 4.8 & 33.3 & 48.4 \\
(256, 2, 32, 128) & 64.7 & 38.4 & \textbf{81.4} & 1.0 & 62.9 & 71.5 & 44.1 & 38.1 & -1.3 & 27.4 & 24.9 \\
(256, 2, 64, 64) & 64.7 & 38.4 & 78.5 & -1.3 & 62.9 & \textbf{82.3} & 51.1 & 37.2 & 4.8 & 51.8 & 42.5 \\
(256, 2, 64, 128) & 64.7 & 38.4 & 78.5 & 1.0 & 62.9 & \textbf{82.3} & 44.1 & 37.2 & -1.3 & 58.7 & 34.5 \\
(256, 2, 128, 64) & 64.7 & 38.4 & 73.8 & -1.3 & 62.9 & \textbf{92.5} & 51.1 & 62.3 & 4.8 & 74.7 & 57.2 \\
(256, 2, 128, 128) & 64.7 & 38.4 & 73.8 & 1.0 & 62.9 & \textbf{92.5} & 44.1 & 62.3 & -1.3 & 57.4 & 37.7 \\
(256, 4, 32, 64) & 64.7 & 26.5 & \textbf{81.4} & -1.3 & 66.1 & 71.5 & 51.1 & 40.8 & 12.2 & 33.3 & 29.6 \\
(256, 4, 32, 128) & 64.7 & 26.5 & \textbf{81.4} & 1.0 & 66.1 & 71.5 & 44.1 & 40.8 & 1.7 & 27.4 & 23.1 \\
(256, 4, 64, 64) & 64.7 & 26.5 & 78.5 & -1.3 & 66.1 & \textbf{82.3} & 51.1 & 46.2 & 12.2 & 51.8 & 41.6 \\
(256, 4, 64, 128) & 64.7 & 26.5 & 78.5 & 1.0 & 66.1 & \textbf{82.3} & 44.1 & 46.2 & 1.7 & 58.7 & 51.5 \\
(256, 4, 128, 64) & 64.7 & 26.5 & 73.8 & -1.3 & 66.1 & \textbf{92.5} & 51.1 & 72.7 & 12.2 & 74.7 & 61.7 \\
(256, 4, 128, 128) & 64.7 & 26.5 & 73.8 & 1.0 & 66.1 & \textbf{92.5} & 44.1 & 72.7 & 1.7 & 57.4 & 50.9 \\
(256, 4, 256, 64) & 64.7 & 26.5 & 69.8 & -1.3 & 66.1 & \textbf{97.7} & 51.1 & 62.5 & 12.2 & 93.8 & 87.5 \\
(256, 4, 256, 128) & 64.7 & 26.5 & 69.8 & 1.0 & 66.1 & \textbf{97.7} & 44.1 & 62.5 & 1.7 & 70.5 & 72.3 \\
(256, 4, 512, 64) & 64.7 & 26.5 & \textbf{96.4} & -1.3 & 66.1 & 96.2 & 51.1 & 87.7 & 12.2 & 93.4 & 81.9 \\
(256, 4, 512, 128) & 64.7 & 26.5 & 96.4 & 1.0 & 66.1 & 96.2 & 44.1 & 87.7 & 1.7 & \textbf{98.4} & 86.7 \\
(512, 1, 32, 64) & 67.1 & 24.2 & 81.4 & -1.3 & 66.8 & \textbf{94.7} & 43.7 & 32.7 & -1.0 & 33.3 & 43.3 \\
(512, 1, 32, 128) & 67.1 & 24.2 & 81.4 & 1.0 & 66.8 & \textbf{94.7} & 50.4 & 32.7 & -1.4 & 27.4 & 34.0 \\
(512, 1, 64, 64) & 67.1 & 24.2 & 78.5 & -1.3 & 66.8 & \textbf{88.7} & 43.7 & 45.0 & -1.0 & 51.8 & 50.0 \\
(512, 1, 64, 128) & 67.1 & 24.2 & 78.5 & 1.0 & 66.8 & \textbf{88.7} & 50.4 & 45.0 & -1.4 & 58.7 & 31.1 \\
(512, 1, 128, 64) & 67.1 & 24.2 & 73.8 & -1.3 & 66.8 & \textbf{99.9} & 43.7 & 59.3 & -1.0 & 74.7 & 53.7 \\
(512, 1, 128, 128) & 67.1 & 24.2 & 73.8 & 1.0 & 66.8 & \textbf{99.9} & 50.4 & 59.3 & -1.4 & 57.4 & 42.8 \\
(512, 2, 32, 64) & 67.1 & 38.4 & 81.4 & -1.3 & 83.4 & \textbf{94.7} & 43.7 & 38.1 & 4.8 & 33.3 & 44.6 \\
(512, 2, 32, 128) & 67.1 & 38.4 & 81.4 & 1.0 & 83.4 & \textbf{94.7} & 50.4 & 38.1 & -1.3 & 27.4 & 41.2 \\
(512, 2, 64, 64) & 67.1 & 38.4 & 78.5 & -1.3 & 83.4 & \textbf{88.7} & 43.7 & 37.2 & 4.8 & 51.8 & 55.8 \\
(512, 2, 64, 128) & 67.1 & 38.4 & 78.5 & 1.0 & 83.4 & \textbf{88.7} & 50.4 & 37.2 & -1.3 & 58.7 & 42.5 \\
(512, 2, 128, 64) & 67.1 & 38.4 & 73.8 & -1.3 & 83.4 & \textbf{99.9} & 43.7 & 62.3 & 4.8 & 74.7 & 67.6 \\
(512, 2, 128, 128) & 67.1 & 38.4 & 73.8 & 1.0 & 83.4 & \textbf{99.9} & 50.4 & 62.3 & -1.3 & 57.4 & 48.8 \\
(512, 4, 32, 64) & 67.1 & 26.5 & 81.4 & -1.3 & 78.6 & \textbf{94.7} & 43.7 & 40.8 & 12.2 & 33.3 & 41.3 \\
(512, 4, 32, 128) & 67.1 & 26.5 & 81.4 & 1.0 & 78.6 & \textbf{94.7} & 50.4 & 40.8 & 1.7 & 27.4 & 29.6 \\
(512, 4, 64, 64) & 67.1 & 26.5 & 78.5 & -1.3 & 78.6 & \textbf{88.7} & 43.7 & 46.2 & 12.2 & 51.8 & 47.7 \\
(512, 4, 64, 128) & 67.1 & 26.5 & 78.5 & 1.0 & 78.6 & \textbf{88.7} & 50.4 & 46.2 & 1.7 & 58.7 & 30.5 \\
(512, 4, 128, 64) & 67.1 & 26.5 & 73.8 & -1.3 & 78.6 & \textbf{99.9} & 43.7 & 72.7 & 12.2 & 74.7 & 48.4 \\
(512, 4, 128, 128) & 67.1 & 26.5 & 73.8 & 1.0 & 78.6 & \textbf{99.9} & 50.4 & 72.7 & 1.7 & 57.4 & 47.6 \\
(512, 4, 256, 64) & 67.1 & 26.5 & 69.8 & -1.3 & 78.6 & \textbf{100.0} & 43.7 & 62.5 & 12.2 & 93.8 & 88.1 \\
(512, 4, 256, 128) & 67.1 & 26.5 & 69.8 & 1.0 & 78.6 & \textbf{100.0} & 50.4 & 62.5 & 1.7 & 70.5 & 52.0 \\
(512, 4, 512, 64) & 67.1 & 26.5 & 96.4 & -1.3 & 78.6 & \textbf{98.5} & 43.7 & 87.7 & 12.2 & 93.4 & 85.5 \\
(512, 4, 512, 128) & 67.1 & 26.5 & 96.4 & 1.0 & 78.6 & \textbf{98.5} & 50.4 & 87.7 & 1.7 & 98.4 & 85.8 \\
\bottomrule
\end{tabular}
\end{table}
