# Supplementary material for: MAVRL: Learning Reward Functions from Multiple Feedback Types with Amortized Variational Inference
Source: arXiv:2602.15206 source file (2026-06-19)
Supplement: Supplementary file 4 [file table_appendix_grid_cliff.tex]

% Requires: \usepackage{booktabs}
\begin{table}[htbp]
\centering
\small
\caption{Full results for Grid Cliff (normalized discounted value, higher is better)}
\label{tab:appendix_grid_cliff}
\begin{tabular}{lrrrr|rrrrrr|r}
\toprule
 & \multicolumn{4}{c|}{Singles} & \multicolumn{6}{c|}{Pairs} & \multicolumn{1}{c}{All} \\
Budget (P,D,R,S) & \fbPref & \fbDemo & \fbRating & \fbStop & \fbDemoPref & \fbPrefRating & \fbPrefStop & \fbDemoRating & \fbDemoStop & \fbRatingStop & \fbPDRS \\
\midrule
(64, 1, 32, 128) & 20.4 & \textbf{62.6} & 19.9 & 8.4 & 16.3 & 27.6 & 38.1 & 32.8 & 56.1 & 29.8 & 51.5 \\
(64, 1, 32, 256) & 20.4 & 62.6 & 19.9 & 37.4 & 16.3 & 27.6 & 60.3 & 32.8 & 72.2 & 63.4 & \textbf{77.8} \\
(64, 1, 64, 128) & 20.4 & 62.6 & 41.3 & 8.4 & 16.3 & 49.5 & 38.1 & 41.8 & 56.1 & 48.6 & \textbf{64.7} \\
(64, 1, 64, 256) & 20.4 & 62.6 & 41.3 & 37.4 & 16.3 & 49.5 & 60.3 & 41.8 & 72.2 & 72.8 & \textbf{90.8} \\
(64, 1, 128, 128) & 20.4 & 62.6 & 75.0 & 8.4 & 16.3 & 73.3 & 38.1 & 63.6 & 56.1 & 59.6 & \textbf{86.6} \\
(64, 1, 128, 256) & 20.4 & 62.6 & 75.0 & 37.4 & 16.3 & 73.3 & 60.3 & 63.6 & 72.2 & 85.6 & \textbf{91.0} \\
(64, 2, 32, 128) & 20.4 & 32.0 & 19.9 & 8.4 & 3.6 & 27.6 & 38.1 & 21.7 & \textbf{52.4} & 29.8 & 39.7 \\
(64, 2, 32, 256) & 20.4 & 32.0 & 19.9 & 37.4 & 3.6 & 27.6 & 60.3 & 21.7 & 72.2 & 63.4 & \textbf{82.3} \\
(64, 2, 64, 128) & 20.4 & 32.0 & 41.3 & 8.4 & 3.6 & 49.5 & 38.1 & 37.6 & \textbf{52.4} & 48.6 & 47.1 \\
(64, 2, 64, 256) & 20.4 & 32.0 & 41.3 & 37.4 & 3.6 & 49.5 & 60.3 & 37.6 & 72.2 & 72.8 & \textbf{86.6} \\
(64, 2, 128, 128) & 20.4 & 32.0 & 75.0 & 8.4 & 3.6 & 73.3 & 38.1 & 73.6 & 52.4 & 59.6 & \textbf{82.2} \\
(64, 2, 128, 256) & 20.4 & 32.0 & 75.0 & 37.4 & 3.6 & 73.3 & 60.3 & 73.6 & 72.2 & 85.6 & \textbf{95.5} \\
(128, 1, 32, 128) & 29.7 & \textbf{62.6} & 19.9 & 8.4 & 29.7 & 38.5 & 38.5 & 32.8 & 56.1 & 29.8 & 51.6 \\
(128, 1, 32, 256) & 29.7 & 62.6 & 19.9 & 37.4 & 29.7 & 38.5 & 60.3 & 32.8 & \textbf{72.2} & 63.4 & 69.0 \\
(128, 1, 64, 128) & 29.7 & \textbf{62.6} & 41.3 & 8.4 & 29.7 & 47.2 & 38.5 & 41.8 & 56.1 & 48.6 & 56.0 \\
(128, 1, 64, 256) & 29.7 & 62.6 & 41.3 & 37.4 & 29.7 & 47.2 & 60.3 & 41.8 & 72.2 & 72.8 & \textbf{73.4} \\
(128, 1, 128, 128) & 29.7 & 62.6 & \textbf{75.0} & 8.4 & 29.7 & 56.0 & 38.5 & 63.6 & 56.1 & 59.6 & 55.9 \\
(128, 1, 128, 256) & 29.7 & 62.6 & 75.0 & 37.4 & 29.7 & 56.0 & 60.3 & 63.6 & 72.2 & \textbf{85.6} & 82.2 \\
(128, 2, 32, 128) & 29.7 & 32.0 & 19.9 & 8.4 & 29.6 & 38.5 & 38.5 & 21.7 & \textbf{52.4} & 29.8 & 42.9 \\
(128, 2, 32, 256) & 29.7 & 32.0 & 19.9 & 37.4 & 29.6 & 38.5 & 60.3 & 21.7 & \textbf{72.2} & 63.4 & 69.0 \\
(128, 2, 64, 128) & 29.7 & 32.0 & 41.3 & 8.4 & 29.6 & 47.2 & 38.5 & 37.6 & 52.4 & 48.6 & \textbf{56.0} \\
(128, 2, 64, 256) & 29.7 & 32.0 & 41.3 & 37.4 & 29.6 & 47.2 & 60.3 & 37.6 & 72.2 & 72.8 & \textbf{77.9} \\
(128, 2, 128, 128) & 29.7 & 32.0 & \textbf{75.0} & 8.4 & 29.6 & 56.0 & 38.5 & 73.6 & 52.4 & 59.6 & 56.0 \\
(128, 2, 128, 256) & 29.7 & 32.0 & 75.0 & 37.4 & 29.6 & 56.0 & 60.3 & 73.6 & 72.2 & 85.6 & \textbf{86.7} \\
(256, 1, 32, 128) & 60.5 & 62.6 & 19.9 & 8.4 & 64.9 & \textbf{69.3} & 60.4 & 32.8 & 56.1 & 29.8 & 69.2 \\
(256, 1, 32, 256) & 60.5 & 62.6 & 19.9 & 37.4 & 64.9 & 69.3 & 73.6 & 32.8 & 72.2 & 63.4 & \textbf{82.3} \\
(256, 1, 64, 128) & 60.5 & 62.6 & 41.3 & 8.4 & 64.9 & 69.3 & 60.4 & 41.8 & 56.1 & 48.6 & \textbf{73.6} \\
(256, 1, 64, 256) & 60.5 & 62.6 & 41.3 & 37.4 & 64.9 & 69.3 & 73.6 & 41.8 & 72.2 & 72.8 & \textbf{86.7} \\
(256, 1, 128, 128) & 60.5 & 62.6 & 75.0 & 8.4 & 64.9 & 78.1 & 60.4 & 63.6 & 56.1 & 59.6 & \textbf{86.8} \\
(256, 1, 128, 256) & 60.5 & 62.6 & 75.0 & 37.4 & 64.9 & 78.1 & 73.6 & 63.6 & 72.2 & \textbf{85.6} & 82.3 \\
(256, 2, 32, 128) & 60.5 & 32.0 & 19.9 & 8.4 & 60.5 & \textbf{69.3} & 60.4 & 21.7 & 52.4 & 29.8 & \textbf{69.3} \\
(256, 2, 32, 256) & 60.5 & 32.0 & 19.9 & 37.4 & 60.5 & 69.3 & \textbf{73.6} & 21.7 & 72.2 & 63.4 & \textbf{73.6} \\
(256, 2, 64, 128) & 60.5 & 32.0 & 41.3 & 8.4 & 60.5 & 69.3 & 60.4 & 37.6 & 52.4 & 48.6 & \textbf{78.1} \\
(256, 2, 64, 256) & 60.5 & 32.0 & 41.3 & 37.4 & 60.5 & 69.3 & 73.6 & 37.6 & 72.2 & 72.8 & \textbf{82.5} \\
(256, 2, 128, 128) & 60.5 & 32.0 & 75.0 & 8.4 & 60.5 & \textbf{78.1} & 60.4 & 73.6 & 52.4 & 59.6 & \textbf{78.1} \\
(256, 2, 128, 256) & 60.5 & 32.0 & 75.0 & 37.4 & 60.5 & 78.1 & 73.6 & 73.6 & 72.2 & \textbf{85.6} & 82.5 \\
\bottomrule
\end{tabular}
\end{table}
