# Supplementary material for: MAVRL: Learning Reward Functions from Multiple Feedback Types with Amortized Variational Inference
Source: arXiv:2602.15206 source file (2026-06-19)
Supplement: Supplementary file 5 [file table_appendix_grid_sparse.tex]

% Requires: \usepackage{booktabs}
\begin{table}[htbp]
\centering
\small
\caption{Full results for Grid Sparse (normalized discounted value, higher is better)}
\label{tab:appendix_grid_sparse}
\begin{tabular}{lrrrr|rrrrrr|r}
\toprule
 & \multicolumn{4}{c|}{Singles} & \multicolumn{6}{c|}{Pairs} & \multicolumn{1}{c}{All} \\
Budget (P,D,R,S) & \fbPref & \fbDemo & \fbRating & \fbStop & \fbDemoPref & \fbPrefRating & \fbPrefStop & \fbDemoRating & \fbDemoStop & \fbRatingStop & \fbPDRS \\
\midrule
(64, 1, 32, 128) & 4.9 & 65.0 & 20.2 & 25.0 & -0.1 & 4.9 & 9.9 & 35.0 & \textbf{80.0} & 40.0 & 30.0 \\
(64, 1, 32, 256) & 4.9 & 65.0 & 20.2 & 35.0 & -0.1 & 4.9 & 45.0 & 35.0 & \textbf{75.0} & 65.0 & 65.0 \\
(64, 1, 64, 128) & 4.9 & 65.0 & 35.0 & 25.0 & -0.1 & 20.0 & 9.9 & 35.0 & \textbf{80.0} & 60.0 & 45.0 \\
(64, 1, 64, 256) & 4.9 & 65.0 & 35.0 & 35.0 & -0.1 & 20.0 & 45.0 & 35.0 & \textbf{75.0} & 65.0 & 70.0 \\
(64, 1, 128, 128) & 4.9 & 65.0 & 75.0 & 25.0 & -0.1 & 30.0 & 9.9 & 50.0 & \textbf{80.0} & \textbf{80.0} & 55.0 \\
(64, 1, 128, 256) & 4.9 & 65.0 & 75.0 & 35.0 & -0.1 & 30.0 & 45.0 & 50.0 & 75.0 & \textbf{85.0} & \textbf{85.0} \\
(64, 2, 32, 128) & 4.9 & 45.5 & 20.2 & 25.0 & -0.1 & 4.9 & 9.9 & 9.9 & \textbf{70.2} & 40.0 & 25.0 \\
(64, 2, 32, 256) & 4.9 & 45.5 & 20.2 & 35.0 & -0.1 & 4.9 & 45.0 & 9.9 & \textbf{85.0} & 65.0 & 60.0 \\
(64, 2, 64, 128) & 4.9 & 45.5 & 35.0 & 25.0 & -0.1 & 20.0 & 9.9 & 30.5 & \textbf{70.2} & 60.0 & 40.0 \\
(64, 2, 64, 256) & 4.9 & 45.5 & 35.0 & 35.0 & -0.1 & 20.0 & 45.0 & 30.5 & \textbf{85.0} & 65.0 & 75.0 \\
(64, 2, 128, 128) & 4.9 & 45.5 & 75.0 & 25.0 & -0.1 & 30.0 & 9.9 & 45.2 & 70.2 & \textbf{80.0} & 55.0 \\
(64, 2, 128, 256) & 4.9 & 45.5 & 75.0 & 35.0 & -0.1 & 30.0 & 45.0 & 45.2 & \textbf{85.0} & \textbf{85.0} & 80.0 \\
(128, 1, 32, 128) & 15.0 & 65.0 & 20.2 & 25.0 & 15.0 & 30.0 & 35.0 & 35.0 & \textbf{80.0} & 40.0 & 40.0 \\
(128, 1, 32, 256) & 15.0 & 65.0 & 20.2 & 35.0 & 15.0 & 30.0 & 50.0 & 35.0 & \textbf{75.0} & 65.0 & 60.0 \\
(128, 1, 64, 128) & 15.0 & 65.0 & 35.0 & 25.0 & 15.0 & 35.0 & 35.0 & 35.0 & \textbf{80.0} & 60.0 & 40.0 \\
(128, 1, 64, 256) & 15.0 & 65.0 & 35.0 & 35.0 & 15.0 & 35.0 & 50.0 & 35.0 & \textbf{75.0} & 65.0 & 60.0 \\
(128, 1, 128, 128) & 15.0 & 65.0 & 75.0 & 25.0 & 15.0 & 45.0 & 35.0 & 50.0 & \textbf{80.0} & \textbf{80.0} & 60.0 \\
(128, 1, 128, 256) & 15.0 & 65.0 & 75.0 & 35.0 & 15.0 & 45.0 & 50.0 & 50.0 & 75.0 & \textbf{85.0} & 70.0 \\
(128, 2, 32, 128) & 15.0 & 45.5 & 20.2 & 25.0 & 9.9 & 30.0 & 35.0 & 9.9 & \textbf{70.2} & 40.0 & 35.0 \\
(128, 2, 32, 256) & 15.0 & 45.5 & 20.2 & 35.0 & 9.9 & 30.0 & 50.0 & 9.9 & \textbf{85.0} & 65.0 & 55.0 \\
(128, 2, 64, 128) & 15.0 & 45.5 & 35.0 & 25.0 & 9.9 & 35.0 & 35.0 & 30.5 & \textbf{70.2} & 60.0 & 40.0 \\
(128, 2, 64, 256) & 15.0 & 45.5 & 35.0 & 35.0 & 9.9 & 35.0 & 50.0 & 30.5 & \textbf{85.0} & 65.0 & 60.0 \\
(128, 2, 128, 128) & 15.0 & 45.5 & 75.0 & 25.0 & 9.9 & 45.0 & 35.0 & 45.2 & 70.2 & \textbf{80.0} & 60.0 \\
(128, 2, 128, 256) & 15.0 & 45.5 & 75.0 & 35.0 & 9.9 & 45.0 & 50.0 & 45.2 & \textbf{85.0} & \textbf{85.0} & 75.0 \\
(256, 1, 32, 128) & 40.0 & 65.0 & 20.2 & 25.0 & 35.0 & 45.0 & 40.0 & 35.0 & \textbf{80.0} & 40.0 & 60.0 \\
(256, 1, 32, 256) & 40.0 & 65.0 & 20.2 & 35.0 & 35.0 & 45.0 & 60.0 & 35.0 & \textbf{75.0} & 65.0 & \textbf{75.0} \\
(256, 1, 64, 128) & 40.0 & 65.0 & 35.0 & 25.0 & 35.0 & 47.3 & 40.0 & 35.0 & \textbf{80.0} & 60.0 & 65.0 \\
(256, 1, 64, 256) & 40.0 & 65.0 & 35.0 & 35.0 & 35.0 & 47.3 & 60.0 & 35.0 & \textbf{75.0} & 65.0 & 70.0 \\
(256, 1, 128, 128) & 40.0 & 65.0 & 75.0 & 25.0 & 35.0 & 50.0 & 40.0 & 50.0 & \textbf{80.0} & \textbf{80.0} & 70.0 \\
(256, 1, 128, 256) & 40.0 & 65.0 & 75.0 & 35.0 & 35.0 & 50.0 & 60.0 & 50.0 & 75.0 & \textbf{85.0} & 75.0 \\
(256, 2, 32, 128) & 40.0 & 45.5 & 20.2 & 25.0 & 40.0 & 45.0 & 40.0 & 9.9 & \textbf{70.2} & 40.0 & 60.0 \\
(256, 2, 32, 256) & 40.0 & 45.5 & 20.2 & 35.0 & 40.0 & 45.0 & 60.0 & 9.9 & \textbf{85.0} & 65.0 & 65.0 \\
(256, 2, 64, 128) & 40.0 & 45.5 & 35.0 & 25.0 & 40.0 & 47.3 & 40.0 & 30.5 & \textbf{70.2} & 60.0 & 60.0 \\
(256, 2, 64, 256) & 40.0 & 45.5 & 35.0 & 35.0 & 40.0 & 47.3 & 60.0 & 30.5 & \textbf{85.0} & 65.0 & 70.0 \\
(256, 2, 128, 128) & 40.0 & 45.5 & 75.0 & 25.0 & 40.0 & 50.0 & 40.0 & 45.2 & 70.2 & \textbf{80.0} & 70.0 \\
(256, 2, 128, 256) & 40.0 & 45.5 & 75.0 & 35.0 & 40.0 & 50.0 & 60.0 & 45.2 & \textbf{85.0} & \textbf{85.0} & 80.0 \\
\bottomrule
\end{tabular}
\end{table}
