# Supplementary material for: MAVRL: Learning Reward Functions from Multiple Feedback Types with Amortized Variational Inference
Source: arXiv:2602.15206 source file (2026-06-19)
Supplement: Supplementary file 6 [file table_appendix_grid_trap.tex]

% Requires: \usepackage{booktabs}
\begin{table}[htbp]
\centering
\small
\caption{Full results for Grid Trap (normalized discounted value, higher is better)}
\label{tab:appendix_grid_trap}
\begin{tabular}{lrrrr|rrrrrr|r}
\toprule
 & \multicolumn{4}{c|}{Singles} & \multicolumn{6}{c|}{Pairs} & \multicolumn{1}{c}{All} \\
Budget (P,D,R,S) & \fbPref & \fbDemo & \fbRating & \fbStop & \fbDemoPref & \fbPrefRating & \fbPrefStop & \fbDemoRating & \fbDemoStop & \fbRatingStop & \fbPDRS \\
\midrule
(64, 1, 32, 128) & 49.7 & 15.6 & 55.3 & -15.2 & 47.1 & 59.2 & 48.9 & 62.3 & \textbf{72.9} & 29.1 & 59.9 \\
(64, 1, 32, 256) & 49.7 & 15.6 & 55.3 & 56.1 & 47.1 & 59.2 & 64.1 & 62.3 & \textbf{69.6} & 67.6 & 64.9 \\
(64, 1, 64, 128) & 49.7 & 15.6 & 60.5 & -15.2 & 47.1 & \textbf{74.2} & 48.9 & 58.3 & 72.9 & 69.0 & 67.1 \\
(64, 1, 64, 256) & 49.7 & 15.6 & 60.5 & 56.1 & 47.1 & 74.2 & 64.1 & 58.3 & 69.6 & 76.2 & \textbf{83.1} \\
(64, 1, 128, 128) & 49.7 & 15.6 & \textbf{91.9} & -15.2 & 47.1 & 81.1 & 48.9 & 79.1 & 72.9 & 78.2 & 82.3 \\
(64, 1, 128, 256) & 49.7 & 15.6 & \textbf{91.9} & 56.1 & 47.1 & 81.1 & 64.1 & 79.1 & 69.6 & 82.5 & 89.2 \\
(64, 2, 32, 128) & 49.7 & 12.6 & 55.3 & -15.2 & 46.1 & 59.2 & 48.9 & 0.9 & 51.4 & 29.1 & \textbf{62.2} \\
(64, 2, 32, 256) & 49.7 & 12.6 & 55.3 & 56.1 & 46.1 & 59.2 & 64.1 & 0.9 & \textbf{73.6} & 67.6 & 66.8 \\
(64, 2, 64, 128) & 49.7 & 12.6 & 60.5 & -15.2 & 46.1 & \textbf{74.2} & 48.9 & 38.7 & 51.4 & 69.0 & 64.1 \\
(64, 2, 64, 256) & 49.7 & 12.6 & 60.5 & 56.1 & 46.1 & 74.2 & 64.1 & 38.7 & 73.6 & 76.2 & \textbf{77.6} \\
(64, 2, 128, 128) & 49.7 & 12.6 & \textbf{91.9} & -15.2 & 46.1 & 81.1 & 48.9 & 72.2 & 51.4 & 78.2 & 72.2 \\
(64, 2, 128, 256) & 49.7 & 12.6 & \textbf{91.9} & 56.1 & 46.1 & 81.1 & 64.1 & 72.2 & 73.6 & 82.5 & 86.5 \\
(128, 1, 32, 128) & 72.2 & 15.6 & 55.3 & -15.2 & 59.5 & \textbf{78.4} & 62.2 & 62.3 & 72.9 & 29.1 & 67.6 \\
(128, 1, 32, 256) & 72.2 & 15.6 & 55.3 & 56.1 & 59.5 & 78.4 & 78.4 & 62.3 & 69.6 & 67.6 & \textbf{86.7} \\
(128, 1, 64, 128) & 72.2 & 15.6 & 60.5 & -15.2 & 59.5 & \textbf{81.1} & 62.2 & 58.3 & 72.9 & 69.0 & 77.6 \\
(128, 1, 64, 256) & 72.2 & 15.6 & 60.5 & 56.1 & 59.5 & 81.1 & 78.4 & 58.3 & 69.6 & 76.2 & \textbf{86.5} \\
(128, 1, 128, 128) & 72.2 & 15.6 & \textbf{91.9} & -15.2 & 59.5 & 83.8 & 62.2 & 79.1 & 72.9 & 78.2 & 81.1 \\
(128, 1, 128, 256) & 72.2 & 15.6 & \textbf{91.9} & 56.1 & 59.5 & 83.8 & 78.4 & 79.1 & 69.6 & 82.5 & 86.5 \\
(128, 2, 32, 128) & 72.2 & 12.6 & 55.3 & -15.2 & 46.1 & \textbf{78.4} & 62.2 & 0.9 & 51.4 & 29.1 & 67.6 \\
(128, 2, 32, 256) & 72.2 & 12.6 & 55.3 & 56.1 & 46.1 & 78.4 & 78.4 & 0.9 & 73.6 & 67.6 & \textbf{83.8} \\
(128, 2, 64, 128) & 72.2 & 12.6 & 60.5 & -15.2 & 46.1 & \textbf{81.1} & 62.2 & 38.7 & 51.4 & 69.0 & 73.0 \\
(128, 2, 64, 256) & 72.2 & 12.6 & 60.5 & 56.1 & 46.1 & 81.1 & 78.4 & 38.7 & 73.6 & 76.2 & \textbf{86.5} \\
(128, 2, 128, 128) & 72.2 & 12.6 & \textbf{91.9} & -15.2 & 46.1 & 83.8 & 62.2 & 72.2 & 51.4 & 78.2 & 83.8 \\
(128, 2, 128, 256) & 72.2 & 12.6 & \textbf{91.9} & 56.1 & 46.1 & 83.8 & 78.4 & 72.2 & 73.6 & 82.5 & 86.5 \\
(256, 1, 32, 128) & 75.7 & 15.6 & 55.3 & -15.2 & 70.3 & \textbf{78.4} & 75.7 & 62.3 & 72.9 & 29.1 & 73.0 \\
(256, 1, 32, 256) & 75.7 & 15.6 & 55.3 & 56.1 & 70.3 & 78.4 & 75.9 & 62.3 & 69.6 & 67.6 & \textbf{81.1} \\
(256, 1, 64, 128) & 75.7 & 15.6 & 60.5 & -15.2 & 70.3 & \textbf{81.1} & 75.7 & 58.3 & 72.9 & 69.0 & 78.4 \\
(256, 1, 64, 256) & 75.7 & 15.6 & 60.5 & 56.1 & 70.3 & \textbf{81.1} & 75.9 & 58.3 & 69.6 & 76.2 & \textbf{81.1} \\
(256, 1, 128, 128) & 75.7 & 15.6 & \textbf{91.9} & -15.2 & 70.3 & 81.1 & 75.7 & 79.1 & 72.9 & 78.2 & 83.8 \\
(256, 1, 128, 256) & 75.7 & 15.6 & \textbf{91.9} & 56.1 & 70.3 & 81.1 & 75.9 & 79.1 & 69.6 & 82.5 & 86.5 \\
(256, 2, 32, 128) & 75.7 & 12.6 & 55.3 & -15.2 & 67.6 & \textbf{78.4} & 75.7 & 0.9 & 51.4 & 29.1 & 73.0 \\
(256, 2, 32, 256) & 75.7 & 12.6 & 55.3 & 56.1 & 67.6 & 78.4 & 75.9 & 0.9 & 73.6 & 67.6 & \textbf{81.1} \\
(256, 2, 64, 128) & 75.7 & 12.6 & 60.5 & -15.2 & 67.6 & \textbf{81.1} & 75.7 & 38.7 & 51.4 & 69.0 & 73.0 \\
(256, 2, 64, 256) & 75.7 & 12.6 & 60.5 & 56.1 & 67.6 & \textbf{81.1} & 75.9 & 38.7 & 73.6 & 76.2 & 78.4 \\
(256, 2, 128, 128) & 75.7 & 12.6 & \textbf{91.9} & -15.2 & 67.6 & 81.1 & 75.7 & 72.2 & 51.4 & 78.2 & 83.8 \\
(256, 2, 128, 256) & 75.7 & 12.6 & \textbf{91.9} & 56.1 & 67.6 & 81.1 & 75.9 & 72.2 & 73.6 & 82.5 & 89.3 \\
\bottomrule
\end{tabular}
\end{table}
