# Supplementary material for: MAVRL: Learning Reward Functions from Multiple Feedback Types with Amortized Variational Inference
Source: arXiv:2602.15206 source file (2026-06-19)
Supplement: Supplementary file 7 [file table_appendix_lunarlander_v3.tex]

% Requires: \usepackage{booktabs}
\begin{table}[htbp]
\centering
\small
\caption{Full results for LunarLander-v3 (normalized return, higher is better)}
\label{tab:appendix_lunarlander_v3}
\begin{tabular}{lrrrr|rrrrrr|r}
\toprule
 & \multicolumn{4}{c|}{Singles} & \multicolumn{6}{c|}{Pairs} & \multicolumn{1}{c}{All} \\
Budget (P,D,R,S) & \fbPref & \fbDemo & \fbRating & \fbStop & \fbDemoPref & \fbPrefRating & \fbPrefStop & \fbDemoRating & \fbDemoStop & \fbRatingStop & \fbPDRS \\
\midrule
(512, 1, 512, 128) & -15.8 & -0.2 & \textbf{23.7} & -30.3 & -3.7 & 11.7 & -15.9 & -38.4 & -59.1 & -11.0 & -2.1 \\
(512, 1, 512, 256) & -15.8 & -0.2 & \textbf{23.7} & -22.2 & -3.7 & 11.7 & 1.4 & -38.4 & -10.4 & 15.1 & 2.0 \\
(512, 1, 1024, 128) & -15.8 & -0.2 & 3.6 & -30.3 & -3.7 & -0.2 & -15.9 & -13.0 & -59.1 & \textbf{11.6} & 2.9 \\
(512, 1, 1024, 256) & -15.8 & -0.2 & 3.6 & -22.2 & -3.7 & -0.2 & 1.4 & -13.0 & -10.4 & \textbf{17.6} & 11.2 \\
(512, 2, 512, 128) & -15.8 & \textbf{108.9} & 23.7 & -30.3 & -12.8 & 11.7 & -15.9 & -16.2 & -25.3 & -11.0 & -7.5 \\
(512, 2, 512, 256) & -15.8 & \textbf{108.9} & 23.7 & -22.2 & -12.8 & 11.7 & 1.4 & -16.2 & -13.9 & 15.1 & 17.5 \\
(512, 2, 1024, 128) & -15.8 & \textbf{108.9} & 3.6 & -30.3 & -12.8 & -0.2 & -15.9 & -1.1 & -25.3 & 11.6 & 10.4 \\
(512, 2, 1024, 256) & -15.8 & \textbf{108.9} & 3.6 & -22.2 & -12.8 & -0.2 & 1.4 & -1.1 & -13.9 & 17.6 & 6.5 \\
(512, 4, 512, 128) & -15.8 & \textbf{113.7} & 23.7 & -30.3 & -29.0 & 11.7 & -15.9 & 8.2 & -34.5 & -11.0 & 12.2 \\
(512, 4, 512, 256) & -15.8 & \textbf{113.7} & 23.7 & -22.2 & -29.0 & 11.7 & 1.4 & 8.2 & 5.0 & 15.1 & 20.2 \\
(512, 4, 1024, 128) & -15.8 & \textbf{113.7} & 3.6 & -30.3 & -29.0 & -0.2 & -15.9 & 8.0 & -34.5 & 11.6 & 7.8 \\
(512, 4, 1024, 256) & -15.8 & \textbf{113.7} & 3.6 & -22.2 & -29.0 & -0.2 & 1.4 & 8.0 & 5.0 & 17.6 & 24.7 \\
(512, 32, 512, 128) & -15.8 & \textbf{115.6} & 23.7 & -30.3 & 39.3 & 11.7 & -15.9 & 42.7 & 39.3 & -11.0 & 59.7 \\
(512, 32, 512, 256) & -15.8 & \textbf{115.6} & 23.7 & -22.2 & 39.3 & 11.7 & 1.4 & 42.7 & 55.7 & 15.1 & 63.4 \\
(512, 32, 1024, 128) & -15.8 & \textbf{115.6} & 3.6 & -30.3 & 39.3 & -0.2 & -15.9 & 38.3 & 39.3 & 11.6 & 71.3 \\
(512, 32, 1024, 256) & -15.8 & \textbf{115.6} & 3.6 & -22.2 & 39.3 & -0.2 & 1.4 & 38.3 & 55.7 & 17.6 & 73.9 \\
(1024, 1, 512, 128) & -3.8 & -0.2 & \textbf{23.7} & -30.3 & 14.3 & -7.1 & -2.6 & -38.4 & -59.1 & -11.0 & 11.8 \\
(1024, 1, 512, 256) & -3.8 & -0.2 & \textbf{23.7} & -22.2 & 14.3 & -7.1 & 1.2 & -38.4 & -10.4 & 15.1 & 7.9 \\
(1024, 1, 1024, 128) & -3.8 & -0.2 & 3.6 & -30.3 & 14.3 & 4.0 & -2.6 & -13.0 & -59.1 & 11.6 & \textbf{16.3} \\
(1024, 1, 1024, 256) & -3.8 & -0.2 & 3.6 & -22.2 & 14.3 & 4.0 & 1.2 & -13.0 & -10.4 & \textbf{17.6} & 8.9 \\
(1024, 2, 512, 128) & -3.8 & \textbf{108.9} & 23.7 & -30.3 & 4.5 & -7.1 & -2.6 & -16.2 & -25.3 & -11.0 & -1.2 \\
(1024, 2, 512, 256) & -3.8 & \textbf{108.9} & 23.7 & -22.2 & 4.5 & -7.1 & 1.2 & -16.2 & -13.9 & 15.1 & 20.5 \\
(1024, 2, 1024, 128) & -3.8 & \textbf{108.9} & 3.6 & -30.3 & 4.5 & 4.0 & -2.6 & -1.1 & -25.3 & 11.6 & 8.5 \\
(1024, 2, 1024, 256) & -3.8 & \textbf{108.9} & 3.6 & -22.2 & 4.5 & 4.0 & 1.2 & -1.1 & -13.9 & 17.6 & -0.3 \\
(1024, 4, 512, 128) & -3.8 & \textbf{113.7} & 23.7 & -30.3 & 11.2 & -7.1 & -2.6 & 8.2 & -34.5 & -11.0 & 8.0 \\
(1024, 4, 512, 256) & -3.8 & \textbf{113.7} & 23.7 & -22.2 & 11.2 & -7.1 & 1.2 & 8.2 & 5.0 & 15.1 & 18.5 \\
(1024, 4, 1024, 128) & -3.8 & \textbf{113.7} & 3.6 & -30.3 & 11.2 & 4.0 & -2.6 & 8.0 & -34.5 & 11.6 & 22.6 \\
(1024, 4, 1024, 256) & -3.8 & \textbf{113.7} & 3.6 & -22.2 & 11.2 & 4.0 & 1.2 & 8.0 & 5.0 & 17.6 & 23.0 \\
(1024, 32, 512, 128) & -3.8 & \textbf{115.6} & 23.7 & -30.3 & 30.0 & -7.1 & -2.6 & 42.7 & 39.3 & -11.0 & 71.0 \\
(1024, 32, 512, 256) & -3.8 & \textbf{115.6} & 23.7 & -22.2 & 30.0 & -7.1 & 1.2 & 42.7 & 55.7 & 15.1 & 77.8 \\
(1024, 32, 1024, 128) & -3.8 & \textbf{115.6} & 3.6 & -30.3 & 30.0 & 4.0 & -2.6 & 38.3 & 39.3 & 11.6 & 67.2 \\
(1024, 32, 1024, 256) & -3.8 & \textbf{115.6} & 3.6 & -22.2 & 30.0 & 4.0 & 1.2 & 38.3 & 55.7 & 17.6 & 80.4 \\
\bottomrule
\end{tabular}
\end{table}
